# Supplementary material for: Intrinsic Orbital Origin for the Chirality-Dependent Nonlinear Planar Hall Effect of Topological Nodal Fermions in Chiral Crystals
Source: arXiv:2405.07529 source file (2024-05-13)
Supplement: Supplementary file 1 [file SM__Chiral_Te_NPHE.pdf]

# Supplemental Material for “Intrinsic Orbital Origin for the Chirality-Dependent Nonlinear Planar Hall Effect of Topological Nodal Fermions in Chiral Crystals”

Mingxiang Pan,[1] Hui Zeng,[2] Erqing Wang,[1] and Huaqing Huang[1,3,4,*]

[1] *School of Physics, Peking University, Beijing 100871, China*
[2] *State Key Laboratory of Low-Dimensional Quantum Physics, Department of Physics, Tsinghua University, Beijing 100084, China*
[3] *Collaborative Innovation Center of Quantum Matter, Beijing 100871, China*
[4] *Center for High Energy Physics, Peking University, Beijing 100871, China*

(Dated: May 13, 2024)

## CONTENTS

I. INPHE from the perspective of the magnetically perturbed INHE 2

II. Construction of the k.p model at H 2

III. Analytic result for a general k.p model around the WP 3
A. Effect of quadratic terms 5
B. Effect of linear tilt terms 6

IV. Comparison with experiment results 8
A. Estimation of $\chi_{xzzx}$ from experimental data 9
B. Extrinsic $\tau^2$ contribution to the nonlinear planar effect 9

V. Model analysis of multifold fermion with high Chern numbers 10
A. Pseudospin-1 10
B. Pseudospin-3/2 11

VI. First-principles calculation methods 12

VII. More calculated results of chiral Te 12

VIII. Topological chiral semimetals with multifold fermions (CoSi, RhSi, RhSn, PtGa, and PtAl) 14

References 19

* Corresponding author: huaqing.huang@pku.edu.cn

## I. INPHE FROM THE PERSPECTIVE OF THE MAGNETICALLY PERTURBED INHE

Based on previous studies [1–3], the intrinsic nonlinear anomalous Hall effect can be expressed as (set $e = \hbar = 1$)

$$\chi^{\rm int}_{abc} = \int [d\boldsymbol{k}] \sum_n f(\epsilon_n)(\partial_b G^n_{ac} - \partial_a G^n_{bc}) \tag{S1}$$

$$= \int [d\boldsymbol{k}] \frac{\partial f(\epsilon_n)}{\partial \epsilon_n} (v^n_a G^n_{bc} - v^n_b G^n_{ac}), \tag{S2}$$

where $v^n_a = \partial\epsilon_n/\partial k_a$ is the band velocity, $G^n_{ab}$ is the Berry-connection polarization (BCP), and the integral is over the BZ with $[d\boldsymbol{k}] \equiv d^3\boldsymbol{k}/(2\pi)^3$. When applying the in-plane magnetic field $B_d$, the INPHE can be derived perturbatively: $\chi^{\rm int}_{abcd} = \partial\chi^{\rm int}_{abc}/\partial B_d$. Therefore, there are two contributions: one is from the perturbation of the BCP: $\partial G^n_{ab}/\partial B_d = \Lambda^n_{abd}$, and the other is from the perturbation on band dispersion: $\partial\epsilon_n/\partial B_d = -\mathcal{M}^n_d$. Specifically, based on Eq. (S2), we derive the first contribution of INPHE from the B-field-induced perturbation of the BCP:

$$\begin{aligned}\chi^{\rm int,I}_{abcd} &= \int [d\boldsymbol{k}] \sum_n \frac{\partial f(\epsilon_n)}{\partial \epsilon_n} \left( v^n_a \frac{\partial G^n_{bc}}{\partial B_d} - v^n_b \frac{\partial G^n_{ac}}{\partial B_d} \right) \\ &= \int [d\boldsymbol{k}] \sum_n \frac{\partial f(\epsilon_n)}{\partial \epsilon_n} \left( v^n_a \Lambda^n_{bcd} - v^n_b \Lambda^n_{acd} \right) \\ &= \int [d\boldsymbol{k}] \sum_n f'(\epsilon_n) \left( v^n_a \Lambda^n_{bcd} - v^n_b \Lambda^n_{acd} \right), \end{aligned} \tag{S3}$$

which is related to the magnetic susceptibility of BCP,

$$\begin{aligned}\Lambda^{n,{\rm S(O)}}_{abc}(\boldsymbol{k}) = 2{\rm Re} \sum_{m\neq n} \Bigg[ & \frac{3 v^{nm}_a v^{mn}_b (\mathcal{M}^{n,{\rm S(O)}}_c - \mathcal{M}^{m,{\rm S(O)}}_c)}{(\epsilon_n - \epsilon_m)^4} \\ & - \sum_{l\neq n} \frac{(v^{lm}_a v^{mn}_b + v^{lm}_b v^{mn}_a)\mathcal{M}^{nl,{\rm S(O)}}_c}{(\epsilon_n - \epsilon_l)(\epsilon_n - \epsilon_m)^3} \\ & - \sum_{l\neq m} \frac{(v^{ln}_a v^{nm}_b + v^{ln}_b v^{nm}_a)\mathcal{M}^{ml,{\rm S(O)}}_c}{(\epsilon_m - \epsilon_l)(\epsilon_n - \epsilon_m)^3} \Bigg]. \end{aligned} \tag{S4}$$

Here $\boldsymbol{\mathcal{M}}^{mn,{\rm S}} = -g\mu_B \boldsymbol{s}^{mn}$ and $\boldsymbol{\mathcal{M}}^{mn,{\rm O}} = \sum_{l\neq n}(\boldsymbol{v}^{ml} + \delta^{lm}\boldsymbol{v}^n) \times \mathcal{A}^{ln}/2$ are the interband spin and orbital magnetic moments, respectively, with $g$ the $g$ factor, $\mu_B$ the Bohr magneton. $\mathcal{A}^{ln}$ is the unperturbed interband Berry connection and $\boldsymbol{s}^{mn}(\boldsymbol{v}^{ml})$ is the spin (velocity) matrix element.

Similarly, based on Eq. (S1), we arrive at the second contribution to the INPHE due to the perturbation on band dispersion:

$$\begin{aligned}\chi^{\rm int,II}_{abcd} &= \int [d\boldsymbol{k}] \sum_n \frac{\partial f(\epsilon_n)}{\partial B_d} \left( \partial_b G^n_{ac} - \partial_a G^n_{bc} \right) \\ &= \int [d\boldsymbol{k}] \sum_n \frac{\partial f(\epsilon_n)}{\partial \epsilon_n} \frac{\partial \epsilon_n}{\partial B_d} \left( \partial_b G^n_{ac} - \partial_a G^n_{bc} \right) \\ &= \int [d\boldsymbol{k}] \sum_n \frac{f(\epsilon_n)}{\partial \epsilon_n} \mathcal{M}^n_d \left( \partial_a G^n_{bc} - \partial_b G^n_{ac} \right) \\ &= \int [d\boldsymbol{k}] \sum_n f'(\epsilon_n) \mathcal{M}^n_d \left( \partial_a G^n_{bc} - \partial_b G^n_{ac} \right), \end{aligned} \tag{S5}$$

which is related to the BCP dipole $\lambda^n_{abc}(\boldsymbol{k}) = \partial_a G^n_{bc} - \partial_b G^n_{ac}$ and magnetic moment $\mathcal{M}^n_d$.

## II. CONSTRUCTION OF THE K.P MODEL AT H

Our first-principles calculations without spin-orbit coupling (SOC) show that the top four valence bands are derived from orbitals with angular momentum $l_z = \pm 1$ [4], while the bottom conduction band is dominated by orbitals with

$l_z = 0$. By including SOC, we find that the bottom conduction bands have a spin splitting near the H points and show a hedgehog spin texture but persist in a band degeneracy at H [5, 6]. The spin-split conduction bands primarily consist of states with total angular momentum $j_z = \pm 1/2$ [5]. Notably, the crystal threefold screw and the twofold rotation symmetries forbid hybridization between the state with $j_z = \pm 1/2$ at H, which protects the WP at H. To construct a low-energy effective model for the spin-split conduction bands around H, we, therefore, take $|s_z = \pm 1/2\rangle$ as a basis. We then derive the k.p Hamiltonian by considering the symmetry constraints using the method of invariants[7]. With basis $|s = \pm 1/2\rangle$, the symmetry operations of the $D_3$ are representations as

$$\begin{aligned} S_{3z} &: \exp\left(-i\pi\sigma_z/3\right), \\ C_{2x} &: -i\sigma_x, \\ T &: -i\sigma_y * K, \end{aligned} \tag{S6}$$

where $K$ is the complex conjugate operator. Using symmetry constraints $\hat{g}(\boldsymbol{k})\hat{H}(\boldsymbol{k})\hat{g}^{-1}(\boldsymbol{k}) = \hat{H}(g \circ \boldsymbol{k})$, we firstly obtain the formula of Hamiltonian keeping up to to the lowest order of $\boldsymbol{k}$. For the right-handed Te, we arrive at a simple Weyl model parameterized by $v_1 = v_2$ and $v_3$,

$$H(\boldsymbol{k}) = v_1(k_x\sigma_x + k_y\sigma_y) + v_3 k_z \sigma_z. \tag{S7}$$

For the left-handed Te, the effective model is similar except for replacing $v_3$ with $-v_3$. Given that the chirality of the WP is determined by the sign of $v_1v_2v_3$, the effective model of right- and left-handed Te have opposite chirality of the WP. Note that the specific formula of the WP in Te is determined by the chiral symmetry. This is different from the Dresselhaus- or Rashba-type formula in conventional polar systems without inversion inversion or mirror symmetry [8]. Consequently, this effective Hamiltonian gives rise to distinct radial spin textures [9].

By further including the second order of $\boldsymbol{k}$, we obtain the effective k.p Hamiltonian for the conduction bands around H in the right-banded Te,

$$H(\boldsymbol{k}) = v_1(k_x\sigma_x + k_y\sigma_y) + v_3 k_z \sigma_z + (c_1(k_x^2 + k_y^2) + c_3 k_z^2)\sigma_0. \tag{S8}$$

In the following, we will analyze the INPHE of chiral Te based on this effective model.

For numerical calculations based on the k.p model, the parameters in Eq. (S8) are set as $v_1 = 0.4415$ eVÅ, $v_3 = 0.5157$ eVÅ, $c_1 = 49.191$ eVÅ$^2$, $c_3 = 68.871$ eVÅ$^2$, which are determined by fitting the band structure with the first-principles calculations. To calculate the INPHE based on the k.p model, we take a $201 \times 201 \times 201$ k-mesh and set the temperature to be $T = 5$ K.

## III. ANALYTIC RESULT FOR A GENERAL K.P MODEL AROUND THE WP

Here, we present analytic results for the intrinsic nonlinear planar Hall effect in a minimal two-band Weyl model, which describes a crossing between two bands. Specifically, the model reads,

$$H_W(\boldsymbol{k}) = v_1 k_x \sigma_x + v_2 k_y \sigma_y + v_3 k_z \sigma_z, \tag{S9}$$

where $\sigma_a$ $(a = x, y, z)$ are Pauli matrices and $v_i$ $(i = 1, 2, 3)$ are band velocities. The energy dispersion is $\varepsilon^{(\pm)}(\boldsymbol{k}) = \pm h = \pm\sqrt{v_1^2k_x^2 + v_2^2k_y^2 + v_3^2k_z^2}$. The Berry curvature of this model is expressed as $\Omega_a^{\pm} = \mp v_1v_2v_3k_a/(2h^3)$ and, therefore, the chirality of this Weyl node is simply given by $\mathcal{C} = \mathrm{sgn}(v_1v_2v_3)$.

After some detailed derivation, we get the BCP tensor:

$$G^{\pm} = \begin{bmatrix} G_{xx} & G_{xz} \\ G_{zx} & G_{zz} \end{bmatrix} = \begin{bmatrix} \pm\frac{v_1^2(v_2^2k_y^2+v_3^2k_z^2)}{4h^5} & \mp\frac{v_1^2v_3^2k_xk_z}{4h^5} \\ \mp\frac{v_1^2v_3^2k_xk_z}{4h^5} & \pm\frac{v_3^2(v_1^2k_x^2+v_2^2k_y^2)}{4h^5} \end{bmatrix}. \tag{S10}$$

Consequently, the BCP dipole is expressed as

$$\lambda_{xzz}^{\pm}(\boldsymbol{k}) = \partial_x G_{zz} - \partial_z G_{xz} = \mp\frac{v_1^2v_3^2k_x}{2h^5}. \tag{S11}$$

The velocity matrix elements are given by

$$
\begin{aligned}
v_x^{\pm} &= \pm\frac{v_1^2 k_x}{h}, \quad v_x^{+-} = (v_x^{-+})^* = \frac{-v_1^2 v_3 k_x k_z - i h v_1 v_2 k_y}{h\sqrt{v_1^2 k_x^2 + v_2^2 k_y^2}}, \\
v_y^{\pm} &= \pm\frac{v_2^2 k_y}{h}, \quad v_y^{+-} = (v_y^{-+})^* = \frac{-v_2^2 v_3 k_y k_z + i h v_1 v_2 k_x}{h\sqrt{v_1^2 k_x^2 + v_2^2 k_y^2}}, \\
v_z^{\pm} &= \pm\frac{v_3^2 k_z}{h}, \quad v_z^{+-} = (v_z^{-+})^* = \frac{v_3\sqrt{v_1^2 k_x^2 + v_2^2 k_y^2}}{h}.
\end{aligned}
\tag{S12}
$$

For the INPHE in the $x$-$z$ plane, the in-plane orbital magnetic moments are given by

$$
\begin{aligned}
\mathcal{M}_x^{\pm,\mathrm{O}} &= -\frac{v_1 v_2 v_3 k_x}{2h^2}, \\
\mathcal{M}_z^{\pm,\mathrm{O}} &= -\frac{v_1 v_2 v_3 k_z}{2h^2},
\end{aligned}
\tag{S13}
$$

both of which are directly related to the chirality $\mathcal{C}$ of the WP and are of the same sign for the two bands ($\pm$). Because the orbital magnetic moment is directly connected to the Berry curvature via $\boldsymbol{\Omega}^{\pm} = \pm\boldsymbol{\mathcal{M}}^{\pm,\mathrm{O}}/h$. The off-diagonal elements $\mathcal{M}^{\pm\mp,\mathrm{O}}$ for the two-band model are just 0 because the two bands have opposite band velocities whose contributions are canceled out exactly. Similarly, we calculate the in-plane spin magnetic moments:

$$
\begin{aligned}
\mathcal{M}_x^{\pm,\mathrm{S}} &= \mp\frac{g\mu_B v_1 k_x}{2h}, \quad \mathcal{M}_x^{\pm\mp,\mathrm{S}} = g\mu_B\frac{v_1 v_3 k_x k_z \pm i h v_2 k_y}{2h\sqrt{v_1^2 k_x^2 + v_2^2 k_y^2}}, \\
\mathcal{M}_z^{\pm,\mathrm{S}} &= \mp\frac{g\mu_B v_3 k_z}{2h}, \quad \mathcal{M}_z^{\pm\mp,\mathrm{S}} = -g\mu_B\frac{\sqrt{v_1^2 k_x^2 + v_2^2 k_y^2}}{2h}.
\end{aligned}
\tag{S14}
$$

Unlike the orbital magnetic moments $\mathcal{M}^{\pm,\mathrm{O}}$, the spin magnetic moments $\mathcal{M}^{\pm,\mathrm{S}}$ have opposite signs for the two bands. Moreover, $\mathcal{M}^{\pm,\mathrm{S}}$ depends on the velocity in their specific direction. In addition, we note that around the WP where $h$ is small, the spin and orbital magnetic moments scale as $k_a/h$ and $k_a/h^2$, respectively. Therefore, the orbital magnetic moment can be more enhanced than the spin magnetic moment with a decreased gap.

The spin and orbital magnetic susceptibility of BCP are given by

$$
\begin{aligned}
\Lambda_{zzx}^{\pm,\mathrm{S}} &= \pm\frac{3v_1 v_3^2 k_x (v_1^2 k_x^2 + v_2^2 k_y^2)}{8h^7} \mp \frac{v_1 v_3^4 k_x k_z^2}{4h^7}, \\
\Lambda_{xzx}^{\pm,\mathrm{S}} &= \mp\frac{v_1^3 v_3^2 k_x^2 k_z}{2h^7} \pm \frac{v_1 v_3^2 k_z (v_3^2 k_z^2 + v_2^2 k_y^2)}{8h^7}, \\
\Lambda_{zzx}^{\pm,\mathrm{O}} &= 0, \quad \Lambda_{xzx}^{\pm,\mathrm{O}} = 0.
\end{aligned}
\tag{S15}
$$

Next, we derive the $xzzx$ element of the conductivity. For simplicity and aesthetics, we omit the subscript ($xzzx$) and move the spin/orbital index (S/O) to subscript for $\alpha$ and $\chi$ hereafter, unless otherwise specified.

$$
\begin{aligned}
\alpha_{\mathrm{S}}^{\mathrm{I},\pm} &= v_x^{\pm}\Lambda_{zzx}^{\pm,\mathrm{S}} - v_z^{\pm}\Lambda_{xzx}^{\pm,\mathrm{S}} = -g\mu_B\left(\frac{3v_1^3 v_3^2 k_x^2 (v_1^2 k_x^2 + v_2^2 k_y^2)}{8h^8} + \frac{v_1^3 v_3^4 k_x^2 k_z^2}{4h^8} - \frac{v_1 v_3^4 k_z^2 (v_2^2 k_y^2 + v_3^2 k_z^2)}{8h^8}\right), \\
\alpha_{\mathrm{S}}^{\mathrm{II},\pm} &= (\partial_x G_{zz} - \partial_z G_{xz})\mathcal{M}_x^{\pm,\mathrm{S}} = g\mu_B\frac{v_1^3 v_3^2 k_x^2}{4h^6}, \\
\alpha_{\mathrm{O}}^{\mathrm{I},\pm} &= v_x^{\pm}\Lambda_{zzx}^{\pm,\mathrm{O}} - v_z^{\pm}\Lambda_{xzx}^{\pm,\mathrm{O}} = 0, \\
\alpha_{\mathrm{O}}^{\mathrm{II},\pm} &= (\partial_x G_{zz} - \partial_z G_{xz})\mathcal{M}_x^{\pm,\mathrm{O}} = \pm\frac{|v_1^3 v_2 v_3^3| k_x^2}{4h^7}\mathrm{sgn}(v_1 v_2 v_3).
\end{aligned}
\tag{S16}
$$

From Eq. (S16) we find that when $h$ is small, $\alpha_{\mathrm{S}}^{\mathrm{I,II}} \propto 1/h^4$ and $\alpha_{\mathrm{O}}^{\mathrm{II}} \propto 1/h^5$. Therefore, $\alpha_{\mathrm{O}}^{\mathrm{II}}$ is the main contribution around the WP. Remarkably, one observes that $\alpha_{\mathrm{S}}^{\mathrm{I},\pm}$ and $\alpha_{\mathrm{S}}^{\mathrm{II},\pm}$ are the same for the two bands ($\pm$) and their signs only rely on the sign of parameter $v_1$. In contrast, $\alpha_{\mathrm{O}}^{\mathrm{II},\pm}$ depends on the chirality of the WP $\mathcal{C} = \mathrm{sgn}(v_1 v_2 v_3)$, implying its

opposite behavior in left- and right-handed Te. Moreover, $\alpha_{\rm O}^{\rm II,\pm}$ has opposite signs for the two bands, which indicate a sign switch when increasing the chemical potential to pass the WP.

For the chiral Te with $D_{3d}$ symmetry, the above model is reduced to $H(\boldsymbol{k}) = v_1(k_x\sigma_x + k_y\sigma_y) + v_3k_z\sigma_z$ in Eq. (S7). To calculate the conductivity, we perform a transformation

$$v_1k_x = h\sin\theta\cos\phi, \quad v_1k_y = h\sin\theta\sin\phi, \quad v_3k_z = h\cos\theta, \tag{S17}$$

and integrate the produce of $f' = -e^{\frac{(\epsilon-\mu)}{k_BT}}/[(1+e^{\frac{(\epsilon-\mu)}{k_BT}})^2k_BT]$ and $\alpha$ [i.e., Eq. (S16)]:

$$\chi_{\rm S}^{\rm I} = -\chi_{\rm S}^{\rm II} = \frac{g\mu_B}{24\pi^2\mu^2}\frac{|v_3|}{v_1}, \tag{S18}$$

$$\chi_{\rm O}^{\rm I} = 0, \tag{S19}$$

$$\chi_{\rm O}^{\rm II} = -\frac{v_3^2\,\mathrm{sgn}\,(v_3)}{24\pi^2\mu^3}. \tag{S20}$$

It is noted that the spin contributions remain the same sign below ($\mu < 0$) and above ($\mu > 0$) the WP. More importantly, the two spin parts with opposite signs cancel out. Therefore, the INPHE conductivity originates primarily from the second part of the orbital contribution ($\chi_{\rm O}^{\rm II}$). Remarkable, the conductivity depends on the chirality of the WP $\mathcal{C} = \mathrm{sgn}(v_3)$ and has opposite signs below ($\mu < 0$) or above ($\mu > 0$) the WP.

In addition, we analyze the $zxxz$ component of the conductivity for comparison. Specifically, we focus on the second part of the orbital contribution

$$\alpha_{zxxz,\rm O}^{\rm II,\pm} = (\partial_zG_{xx} - \partial_xG_{zx})\mathcal{M}_z^{\pm,\rm O} = \pm\frac{|v_1^3v_2v_3^3|k_z^2}{4h^7}\mathrm{sgn}(v_1v_2v_3), \tag{S21}$$

which is similar to $\alpha_{xzzx,\rm O}^{\rm II,\pm}$ in Eq. (S5) with $k_x$ being replaced by $k_z$.

### A. Effect of quadratic terms

To further consider the quadratic dispersion of the conduction bands around the H point, we add the following quadratic term to the above Hamilton (S9), which is allowed in the $D_{3d}$ symmetry of the chiral Te,

$$H_{\rm quad}(\boldsymbol{k}) = c_1k_x^2 + c_2k_y^2 + c_3k_z^2. \tag{S22}$$

The band dispersion of the two bands becomes $\epsilon^{(\pm)}(\boldsymbol{k}) = c_1k_x^2 + c_2k_y^2 + c_3k_z^2 \pm h$. The BCP elements and the velocity matrix elements are given by

$$G_{zz} = \pm\frac{v_3^2(v_1^2k_x^2 + v_2^2k_y^2)}{4h^5}, \quad G_{xz} = \mp\frac{v_1^2v_3^2k_xk_z}{4h^5}, \quad \partial_xG_{zz} - \partial_zG_{xz} = \mp\frac{v_1^2v_3^2k_x}{2h^5}; \tag{S23}$$

$$\begin{aligned} v_x^{\pm} &= \pm\frac{v_1^2k_x}{h} + 2c_1k_x, \quad v_x^{+-} = (v_x^{-+})^* = \frac{-v_1^2v_3k_xk_z - ihv_1v_2k_y}{h\sqrt{v_1^2k_x^2 + v_2^2k_y^2}}, \\ v_y^{\pm} &= \pm\frac{v_2^2k_y}{h} + 2c_2k_y, \quad v_y^{+-} = (v_y^{-+})^* = \frac{-v_2^2v_3k_yk_z + ihv_1v_2k_x}{h\sqrt{v_1^2k_x^2 + v_2^2k_y^2}}, \\ v_z^{\pm} &= \pm\frac{v_3^2k_z}{h} + 2c_3k_z, \quad v_z^{+-} = (v_z^{-+})^* = \frac{v_3\sqrt{v_1^2k_x^2 + v_2^2k_y^2}}{h}. \end{aligned} \tag{S24}$$

It is noted that only the diagonal elements of the velocity matrix are affected by the quadratic term. The orbital magnetic moments are modified as

$$\begin{aligned} \mathcal{M}_x^{\pm,\rm O} &= -\frac{v_1v_2v_3k_x}{2h^2}, \\ \mathcal{M}_x^{\pm\mp,\rm O} &= -\frac{c_3v_1v_2k_xk_z}{h\sqrt{v_1^2k_x^2 + v_2^2k_y^2}} \mp \frac{ic_2v_3k_y\sqrt{v_1^2k_x^2 + v_2^2k_y^2}}{h^2} \mp \frac{ic_3v_2^2v_3k_yk_z^2}{h^2\sqrt{v_1^2k_x^2 + v_2^2k_y^2}}. \end{aligned} \tag{S25}$$

The diagonal element is the same as Eq. (S13), but the off-diagonal element does not vanish anymore. Therefore, the second part of the orbital contribution to conductivity remains the same as that without the quadratic term [i.e., Eq. (S16)]:

$$\alpha_{\mathrm{O}}^{\mathrm{II},\pm} = (\partial_x G_{zz} - \partial_z G_{xz})\mathcal{M}_x^{\pm,\mathrm{O}} = \pm\frac{|v_1^3 v_2 v_3^3| k_x^2}{4h^7}\mathrm{sgn}(v_1 v_2 v_3). \tag{S26}$$

Now, we analyze the first part of the orbital contribution which does not vanish anymore

$$\begin{aligned}
\Lambda_{zzx}^{\pm,\mathrm{O}} &= \mp\frac{c_3 v_1 v_2 v_3^3 k_x k_z^2}{2h^7},\\
\Lambda_{xzx}^{\pm,\mathrm{O}} &= \mp\frac{c_3 v_1^3 v_2 v_3 k_x^2 k_z}{4h^7} \pm \frac{v_1 v_2 v_3^3 k_z (c_2 k_y^2 + c_3 k_z^2)}{4h^7},\\
\alpha_{\mathrm{O}}^{\mathrm{I},\pm} &= v_x^{\pm}\Lambda_{zzx}^{\pm,\mathrm{O}} - v_z^{\pm}\Lambda_{xzx}^{\pm,\mathrm{O}}\\
&= -\frac{v_1 v_2 v_3^5 k_z^2 (c_2 k_y^2 + c_3 k_z^2)}{4h^8} - \frac{c_3 v_1^3 v_2 v_3^3 k_x^2 k_z^2}{4h^8} \mp \frac{c_1 c_3 v_1 v_2 v_3^3 k_x^2 k_z^2}{h^7}\\
&\quad \pm \frac{c_3^2 v_1^3 v_2 v_3 k_x^2 k_z^2}{2h^7} \mp \frac{c_3 v_1 v_2 v_3^3 k_z^2 (c_2 k_y^2 + c_3 k_z^2)}{2h^7}.
\end{aligned} \tag{S27}$$

Roughly speaking, $\alpha_{\mathrm{O}}^{\mathrm{I},\pm}$ scales as $1/h^{3\sim 4}$ around the WP, which should make a small contribution to the conductivity compared to $\alpha_{\mathrm{O}}^{\mathrm{II},\pm}$.

Similarly, we derive the spin magnetic moment and the second part of the spin contribution

$$\mathcal{M}_x^{\pm,\mathrm{S}} = \mp g\mu_B \frac{v_1 k_x}{2h}, \tag{S28}$$

$$\alpha_{\mathrm{S}}^{\mathrm{II},\pm} = (\partial_x G_{zz} - \partial_z G_{xz})\mathcal{M}_x^{\pm,\mathrm{S}} = g\mu_B \frac{v_1^3 v_3^2 k_x^2}{4h^6}, \tag{S29}$$

which remain the same as the results in the absence of the quadratic term [i.e., Eq. (S13) and (S16)]. However, the first part of the spin contribution becomes complicated,

$$\begin{aligned}
\Lambda_{zzx}^{\pm,\mathrm{S}} &= -g\mu_B\left(\pm\frac{3v_1 v_3^2 k_x (v_1^2 k_x^2 + v_2^2 k_y^2)}{8h^7} \mp \frac{v_1 v_3^4 k_x k_z^2}{4h^7}\right),\\
\Lambda_{xzx}^{\pm,\mathrm{S}} &= -g\mu_B\left(\mp\frac{v_1^3 v_3^2 k_x^2 k_z}{2h^7} \pm \frac{v_1 v_3^2 k_z (v_3^2 k_z^2 + v_2^2 k_y^2)}{8h^7}\right),\\
\alpha_{\mathrm{S}}^{\mathrm{I},\pm} &= v_x^{\pm}\Lambda_{zzx}^{\pm,\mathrm{S}} - v_z^{\pm}\Lambda_{xzx}^{\pm,\mathrm{S}}\\
&= -g\mu_B\left[\frac{3v_1^3 v_3^2 k_x^2 (v_1^2 k_x^2 + v_2^2 k_y^2)}{8h^8} + \frac{v_1^3 v_3^4 k_x^2 k_z^2}{4h^8} - \frac{v_1 v_3^4 k_z^2 (v_2^2 k_y^2 + v_3^2 k_z^2)}{8h^8}\right.\\
&\quad \left.\pm\frac{3c_1 v_1 v_3^2 k_x^2 (v_1^2 k_x^2 + v_2^2 k_y^2)}{4h^7} \mp \frac{c_1 v_1 v_3^4 k_x^2 k_z^2}{2h^7} \pm \frac{c_3 v_1^3 v_3^2 k_x^2 k_z^2}{h^7} \mp \frac{c_3 v_1 v_3^2 k_z^2 (v_3^2 k_z^2 + v_2^2 k_y^2)}{4h^7}\right].
\end{aligned} \tag{S30}$$

It is noted that the spin magnetic susceptibility $\Lambda_{abc}^{n}$ remains unchanged. However, due to the modification on the velocity matrix element, some extra terms that are induced by the quadratic term appear in $\alpha_{\mathrm{S}}^{\mathrm{I},\pm}$, i.e., the last line in Eq. (S27).

### B. Effect of linear tilt terms

Now, let's consider the effect of linear tilt terms which can be introduced by applying external strain to the chiral Te. Specifically, we add the following linear tilt term to Eq. (S9):

$$\tilde{H}_{tilt}(\boldsymbol{k}) = w_1 k_x + w_2 k_y + w_3 k_z. \tag{S31}$$

This term does not change $\alpha^{\mathrm{II,O}}$ and $\alpha^{\mathrm{II,S}}$, but make $\alpha_{\mathrm{O}}^{\mathrm{I}}$ have the same magnitude as $\alpha_{\mathrm{O}}^{\mathrm{II}}$. The major change is that The BCP element and the velocity matrix elements are given by

$$G_{zz} = \pm\frac{v_3^2 (v_1^2 k_x^2 + v_2^2 k_y^2)}{4h^5}, \quad G_{xz} = \mp\frac{v_1^2 v_3^2 k_x k_z}{4h^5}, \quad \partial_x G_{zz} - \partial_z G_{xz} = \mp\frac{v_1^2 v_3^2 k_x}{2h^5}; \tag{S32}$$

$$\begin{aligned}
v_x^{\pm} &= \pm\frac{v_1^2 k_x}{h} + w_1, \quad v_x^{+-} = (v_x^{-+})^* = \frac{-v_1^2 v_3 k_x k_z - ihv_1 v_2 k_y}{h\sqrt{v_1^2 k_x^2 + v_2^2 k_y^2}},\\
v_y^{\pm} &= \pm\frac{v_2^2 k_y}{h} + w_2, \quad v_y^{+-} = (v_y^{-+})^* = \frac{-v_2^2 v_3 k_y k_z + ihv_1 v_2 k_x}{h\sqrt{v_1^2 k_x^2 + v_2^2 k_y^2}},\\
v_z^{\pm} &= \pm\frac{v_3^2 k_z}{h} + w_3, \quad v_z^{+-} = (v_z^{-+})^* = \frac{v_3\sqrt{v_1^2 k_x^2 + v_2^2 k_y^2}}{h}.
\end{aligned} \tag{S33}$$

It is noted that only the diagonal elements of the velocity matrix are affected by the linear term. In contrast, the diagonal element of the orbital magnetic moment remains the same, but the off-diagonal elements are no longer zero:

$$\begin{aligned}
\mathcal{M}_x^{\pm,\mathrm{O}} &= -\frac{v_1 v_2 v_3 k_x}{2h^2},\\
\mathcal{M}_x^{\pm\mp,\mathrm{O}} &= \mp\frac{iw_2 v_3\sqrt{v_1^2 k_x^2 + v_2^2 k_y^2}}{2h^2} - w_3\frac{hv_1 v_2 k_x \pm iv_2^2 v_3 k_y k_z}{2h^2\sqrt{v_1^2 k_x^2 + v_2^2 k_y^2}}.
\end{aligned} \tag{S34}$$

The second part of the orbital contribution still remains unchanged,

$$\alpha_{\mathrm{O}}^{\mathrm{II},\pm} = (\partial_x G_{zz} - \partial_z G_{xz})\mathcal{M}_x^{\pm,\mathrm{O}} = \pm\frac{|v_1^3 v_2 v_3^3|k_x^2}{4h^7}\mathrm{sgn}(v_1 v_2 v_3). \tag{S35}$$

In contrast, for the first part of the orbital contribution, we get

$$\begin{aligned}
\Lambda_{zzx}^{\pm,\mathrm{O}} &= \mp\frac{w_3 v_1 v_2 v_3^3 k_x k_z}{4h^7},\\
\Lambda_{xzx}^{\pm,\mathrm{O}} &= \mp\frac{w_3 v_1^3 v_2 v_3 k_x^2}{8h^7} \pm \frac{v_1 v_2 v_3^3 k_z (w_2 k_y + w_3 k_z)}{8h^7},
\end{aligned} \tag{S36}$$

and

$$\begin{aligned}
\alpha_{\mathrm{O}}^{\mathrm{I},\pm} =& v_x^{\pm}\Lambda_{zzx}^{\pm,\mathrm{O}} - v_z^{\pm}\Lambda_{xzx}^{\pm,\mathrm{O}}\\
=& -\frac{v_1 v_2 v_3^5 k_z^2 (w_2 k_y + w_3 k_z)}{8h^8} - \frac{w_3 v_1^3 v_2 v_3^3 k_x^2 k_z}{8h^8}\\
&\mp\frac{w_1 w_3 v_1 v_2 v_3^3 k_x k_z}{4h^7} \pm \frac{w_3^2 v_1^3 v_2 v_3 k_x^2}{8h^7} \mp \frac{w_3 v_1 v_2 v_3^3 k_z (w_2 k_y + w_3 k_z)}{8h^7}.
\end{aligned} \tag{S37}$$

As shown in Eq. (S37), $\alpha_{\mathrm{O}}^{\mathrm{I}} \propto 1/h^5$, which is the same as $\alpha_{\mathrm{O}}^{\mathrm{II}}$. The 3% strain adds three Weyl nodes around the H point whose chirality is -1. We find that $w_3 \approx 0$ for these Weyl nodes, So the band is symmetric about $k_z$, which means only $k_z$-even terms are necessary and we can omit terms having $w_3$. So only one term is left:

$$\alpha_{\mathrm{O,tilt}}^{\mathrm{I},\pm} = -\frac{w_2 k_y |v_1 v_2 v_3^5| k_z^2}{8h^8}\mathrm{sgn}(v_1 v_2 v_3). \tag{S38}$$

Then we calculate the INPHE conductivity $\chi_{\mathrm{O,tilt}}^{\mathrm{I}}$by integrating the produte of $f'$ and $\alpha_{\mathrm{O,tilt}}^{\mathrm{I},\pm}$ in (S38). To simplify the calculations, we neglect the $w_1$ term in the Hamiltonian. By applying a coordinate transformation similar to that described in Eq. (S17), we can get

$$\begin{aligned}
\chi_{\mathrm{O,tilt}}^{\mathrm{I}} &= \int [d\boldsymbol{k}]\delta(\mu - w_2 k_y \mp h)\frac{w_2|v_1 v_2 v_3^3|\cos^2\theta\sin\theta\sin\phi}{8v_2 h^5}\mathrm{sgn}(v_1 v_2 v_3)\\
&= \int\frac{d\theta d\phi}{(2\pi)^3}\frac{w_2 v_3^2\cos^2\theta\sin^2\theta\sin\phi}{8v_2|\mu|^3}(\frac{w_2}{v_2}\sin\theta\sin\phi \pm 1)^2\Theta[\mu/(\frac{w_2}{v_2}\sin\theta\sin\phi \pm 1)]\mathrm{sgn}(v_1 v_2 v_3).
\end{aligned} \tag{S39}$$

In the above equation, we assume summation over two bands and $\Theta[cdot]$ represents the Heaviside step function. To determine the range of the integral, one needs to discuss the variable in $\Theta$ under separate situations. When $|w_2| < |v_2|$, the sign of $\frac{w_2}{v_2}\sin\theta\sin\phi \pm 1$ is entirely determined by the sign preceding the number 1, so we can easily get

$$\begin{aligned}
\chi_{\mathrm{O,tilt}}^{\mathrm{I}} &= \int\frac{d\theta d\phi}{(2\pi)^3}\frac{w_2 v_3^2\cos^2\theta\sin^2\theta\sin\phi}{8v_2|\mu|^3}(\frac{w_2}{v_2}\sin\theta\sin\phi + \mathrm{sgn}(\mu))^2\mathrm{sgn}(v_1 v_2 v_3)\\
&= \frac{w_2^2}{v_2^2}\frac{v_3^2}{120\pi^2\mu^3}\mathrm{sgn}(v_1 v_2 v_3) \propto \mathcal{C}/\mu^3.
\end{aligned} \tag{S40}$$

Next, we consider the case where $|w_2| \gg |v_2|$. In this case,

$$\mathrm{sgn}(\frac{w_2}{v_2}\sin\theta\sin\phi \pm 1) \approx \mathrm{sgn}(\frac{w_2}{v_2}\sin\theta\sin\phi) = \mathrm{sgn}(\frac{w_2}{v_2})\mathrm{sgn}(\sin\phi). \tag{S41}$$

Then

$$\begin{aligned}\chi^{\mathrm{I}}_{\mathrm{O,tilt}} \approx& \int \frac{d\theta d\phi}{(2\pi)^3}\frac{|w_2|v_3^2\cos^2\theta\sin^2\theta|\sin\phi|}{8|v_2|\mu^3}(\frac{w_2}{v_2}\sin\theta\sin\phi\pm 1)^2\mathrm{sgn}(v_1v_2v_3)\\ =& 2\int \frac{d\theta}{(2\pi)^3}\frac{|w_2|v_3^2\cos^2\theta\sin^2\theta}{8|v_2|\mu^3}(\frac{4}{3}(\frac{w_2}{v_2})^2\sin^2\theta + 2)\mathrm{sgn}(v_1v_2v_3)\\ =& |\frac{w_2}{v_2}|\frac{v_3^2}{128\pi^2\mu^3}(1+\frac{w_2^2}{3v_2^2})\mathrm{sgn}(v_1v_2v_3) \propto \mathcal{C}/\mu^3,\end{aligned} \tag{S42}$$

where the factor of 2 in the second line arises because in the limit case considered, the two bands nearly overlap, thus contributing equally. Based on the above analysis, we conclude that $\chi^{\mathrm{I}}_{\mathrm{O,tilt}} \propto \mathcal{C}/\mu^3$ in both type-I weak-tilted and type-II overtilted WPs.

In addition, we also derive the spin contributions in the presence of the linear term. The spin magnetic moment and the second part of the spin contribution remain unchanged,

$$M_x^{\pm,\mathrm{S}} = \mp g\mu_B\frac{v_1k_x}{2h}, \tag{S43}$$

$$\alpha_{\mathrm{S}}^{\mathrm{II},\pm} = (\partial_x G_{zz} - \partial_z G_{xz})\mathcal{M}_x^{\pm,\mathrm{S}} = g\mu_B\frac{v_1^3v_3^2k_x^2}{4h^6}. \tag{S44}$$

We analyze the first part of the spin contribution

$$\begin{aligned}\Lambda_{zzx}^{\pm,\mathrm{S}} =& -g\mu_B\left(\pm\frac{3v_1v_3^2k_x(v_1^2k_x^2+v_2^2k_y^2)}{8h^7}\mp\frac{v_1v_3^4k_xk_z^2}{4h^7}\right),\\ \Lambda_{xzx}^{\pm,\mathrm{S}} =& -g\mu_B\left(\mp\frac{v_1^3v_3^2k_x^2k_z}{2h^7}\pm\frac{v_1v_3^2k_z(v_3^2k_z^2+v_2^2k_y^2)}{8h^7}\right),\\ \alpha_{\mathrm{S}}^{\mathrm{I},\pm} =& v_x^{\pm}\Lambda_{zzx}^{\pm,\mathrm{S}} - v_z^{\pm}\Lambda_{xzx}^{\pm,\mathrm{S}}\\ =& -g\mu_B\left[\frac{3v_1^3v_3^2k_x^2(v_1^2k_x^2+v_2^2k_y^2)}{8h^8}+\frac{v_1^3v_3^4k_x^2k_z^2}{4h^8}-\frac{v_1v_3^4k_z^2(v_2^2k_y^2+v_3^2k_z^2)}{8h^8}\right.\\ &\left.+w_1(\pm\frac{3v_1v_3^2k_x(v_1^2k_x^2+v_2^2k_y^2)}{8h^7}\mp\frac{v_1v_3^4k_xk_z^2}{4h^7})-w_3(\mp\frac{v_1^3v_3^2k_x^2k_z}{2h^7}\pm\frac{v_1v_3^2k_z(v_3^2k_z^2+v_2^2k_y^2)}{8h^7})\right].\end{aligned} \tag{S45}$$

where the last line of $\alpha_{\mathrm{S}}^{\mathrm{I},\pm}$ is the modification induced by the linear term.

## IV. COMPARISON WITH EXPERIMENT RESULTS

In a recent transport experiment on chiral Te [10], the nonlinear planar Hall conductivity has been measured with an alternating current applied along the Te atomic chain direction (i.e., $\theta = 0$) [10]. According to Eq. (5) in the main text, $\chi_{\mathrm{H}}^{\mathrm{int}} = \chi_{xzzx}\sin(\phi)$ coincide with the experimentally observed conductivity which follows a cosine angular dependence on the $B$-field direction with $2\pi$-periodicity and reaches maximum (vanishes) when $B$ is orthogonal (parallel) to the current direction. Moreover, the opposite chirality dependence of the conductivity, strong enhancement around the band edge, and sign inversion crossing the WP agree well with the opposite gate-tunable nonlinear planar Hall response between left- and right-handed Te in experiments.

Nevertheless, the amplitude of the experimental values, as estimated below in Sec. IV A, is at least one order of magnitude smaller than our calculation show in Fig. 1(f,g). Several factors could play a role here, including the highly sensitive thickness, temperature, and doping dependence of the INPHE [11–13]. Beyond the intrinsic contribution, we also estimate other extrinsic contributions that depend on scattering (see Sec. IV B), and found that they are orders of magnitude smaller than the experimental values, indicating that INPHE is the primary mechanism. More investigations are needed to distinguish various mechanisms by their different scaling with $\tau$ (e.g., by plotting the NPHE conductivity against the linear longitudinal conductivity) [14].

### A. Estimation of $\chi_{xzzx}$ from experimental data

For the experimental measurements of chiral Te conducted recently [10], we derive the corresponding $\chi_{xzzx}$ based on the following expression [15],

$$\chi_{xzzx} = -2\sigma_{zz}\frac{L^2}{WB}\frac{V_{zx}^{(2\omega)}}{V_{zz}^2} = \chi^{l,r}\left[-2\sigma_{zz}\frac{L^2}{WR_{zz}^2}\right], \tag{S46}$$

where $B$ is the magnetic field strength, $L$ and $W$ are the typical length and width of the Hall bar structure, respectively. $V_{zz}$ and $V_{zx}^{(2\omega)}$ are the measured first and second harmonic voltage signals in the longitudinal and transverse directions. Here $\chi^{l,r}$ describes the strength of the nonlinear planar Hall effect in experiments reported in Ref. [10] and is defined as $V_{zx}^{(2\omega)l,r}(B,I) = \chi^{l,r}BI^2$ with superscript $(l,r)$ denoting the left- and right-banded Te. In the constant relaxation-time approximation, the longitudinal linear conductivity $\sigma_{zz}$ is estimated as

$$\sigma_{zz} = \tau\frac{e^2}{4\pi^3}\sum_n\int d\boldsymbol{k}\,(v_{z,n}(\boldsymbol{k}))^2\left(-\frac{\partial f}{\partial\epsilon}\right)_{\epsilon=\epsilon_n(\boldsymbol{k})} = \tau\frac{e^2}{\hbar^2}\int[d\boldsymbol{k}]\sum_n\left(\frac{\partial\epsilon_n(\boldsymbol{k})}{\partial k_z}\right)^2\left(-\frac{\partial f}{\partial\epsilon}\right)_{\epsilon=\epsilon_n(\boldsymbol{k})}. \tag{S47}$$

Taking a typical relaxation time $\tau \approx 0.05$ ps, our calculations yield a $\sigma_{zz}$ approximately on the order of $5\times10^4\ \Omega^{-1}\text{m}^{-1}$. By substituting in the experimental data, $B = 18$ T, $L = 20$ $\mu$m, $W = 15$ $\mu$m, $V_{zz} \approx 6$ mV, and $V_{zx}^{(2\omega)} \approx 1$ $\mu$V, we estimate that the experimental value of $\chi_{xzzx}$ is approximately on the order of $10^{-2}$ AV$^{-2}$T$^{-1}$, which is about one order of magnitude smaller than our theoretical calculations. Several factors could play a role in diminishing experimental values, including the thickness of the sample, the highly sensitive doping, and the temperature dependence of the INPHE. More investigations are needed for a quantitative comparison between our theory and the experiment.

### B. Extrinsic $\tau^2$ contribution to the nonlinear planar effect

In addition to the intrinsic NPHE, we also estimate the extrinsic contributions that scale as $\tau^2$. The extrinsic contributions include the Zeeman and Berry curvature terms, which are given by [16–18]

$$\chi_{abcd}^{(2),Z} = \tau^2\int[d\mathbf{k}]\alpha_{abcd}^{(2)}f_0' = \tau^2\int[d\mathbf{k}][v_{abc}\mathcal{M}_d - v_c\partial_{ab}\mathcal{M}_d]f_0', \tag{S48}$$

$$\begin{aligned}\chi_{abcd}^{(2),\Omega} = \tau^2\int[d\mathbf{k}]\alpha_{abcd}^{(2),\Omega}f_0' =& \tau^2\int[d\mathbf{k}]\,[2(v_{ab}v_c\Omega_d + v_av_c\partial_b\Omega_d) - 2\delta_{cd}v_{ae}v_b\Omega_e \\ & -\delta_{ad}(v_{be}v_c\Omega_e + v_cv_e\partial_b\Omega_e) + \delta_{dc}v_av_e\partial_b\Omega_e - v_av_c\partial_b\Omega_d]\,f_0',\end{aligned} \tag{S49}$$

where $\partial_a = \partial_{k_a}, \partial_{ab} = \partial_{k_a}\partial_{k_b}$, $v_a = \partial_a\epsilon_{\boldsymbol{k}}$, $v_{ab} = \partial_{ab}\epsilon_{\boldsymbol{k}}$ and $v_{abc} = \partial_a\partial_b\partial_c\epsilon_{\boldsymbol{k}}$. $\mathcal{M}_d$ denotes the magnetic moment including spin and orbital parts. The first term is attributed to the $\boldsymbol{B}$ field-induced perturbation to the band structure (modification of $\epsilon_{\boldsymbol{k}}$) by the Zeeman coupling to the spin and orbital magnetic moments of Bloch states. The second term comes from the modified density of states and anomalous velocity induced by Berry curvature.

Using the model described by Eq.(15) and the parameters in the main text, we obtain the $xzzx$ element:

$$\alpha_{\text{S}}^{(2),\pm} = -g\mu_B\left(-\frac{v_1^3v_3^2k_x^2}{2h^4} + \frac{v_1v_3^4k_z^2}{2h^4} \pm \frac{2c_3v_1v_3^2k_z^2}{h^3} \mp \frac{3c_3v_1^3v_3^2k_x^2k_z^2}{h^5}\right), \tag{S50}$$

$$\alpha_{\text{O}}^{(2),\pm} = \pm\frac{v_1^3v_2v_3^3k_x^2}{2h^5} \mp \frac{v_1v_2v_3^5k_z^2}{h^5} \pm \frac{5v_1^3v_2v_3^5k_x^2k_z^2}{2h^7} - \frac{2c_3v_1v_2v_3^3k_z^2}{h^4} + \frac{8c_3v_1^3v_2v_3^3k_x^2k_z^2}{h^6}, \tag{S51}$$

$$\begin{aligned}\alpha^{(2),\Omega,\pm} =& \mp\frac{v_1^3v_2v_3^5k_x^2k_z^2}{2h^7} - \frac{c_3v_1^3v_2v_3^3k_x^2k_z^2}{h^6} \pm \frac{2v_1v_2^3v_3^5k_y^2k_z^2}{h^7} \pm \frac{6c_2c_3v_1v_2v_3^3k_y^2k_z^2}{h^5} + \frac{v_1v_2v_3^3k_y^2k_z^2(3c_2v_3^2+4c_3v_2^2)}{h^6} \\ & \left(\mp\frac{v_1v_2v_3^5}{h^5} \mp \frac{4c_3^2v_1v_2v_3}{h^3} - \frac{4c_3v_1v_2v_3^3}{h^4}\right)k_z^2 + \left(\pm\frac{2v_1v_2v_3^7}{h^7} \pm \frac{6c_3^2v_1v_2v_3^3}{h^5} + \frac{7c_3v_1v_2v_3^5}{h^6}\right)k_z^4.\end{aligned} \tag{S52}$$

It is clear that when $h$ is small, $\alpha_{\text{S}}^{(2),\pm} \propto 1/h^2$, $\alpha_{\text{O}}^{(2),\pm} \propto 1/h^3$ and $\alpha^{(2),\Omega,\pm} \propto 1/h^3$, which is less significant than the intrinsic contributions with a decreased gap around the WP. Taking a typical relaxation time $\tau \approx 0.01 \sim 0.1$ ps[19], the estimated extrinsic contribution is on the order of $10^{-3} \sim 10^{-5}$ AV$^{-2}$T$^{-1}$, which is smaller than the experimental values. In experiments, the extrinsic contribution can be separated from the intrinsic one according to their different scaling with $\tau$, for example, by plotting against the linear longitudinal conductivity.

## V. MODEL ANALYSIS OF MULTIFOLD FERMION WITH HIGH CHERN NUMBERS

Multifold fermions can be described by Hamiltonians with pseudo-spin $S$, where $S=(N-1)/2$. Specifically, the case of $S=1/2$ corresponds to the model presented in Appendix C. The generic Hamiltonian with pseudo-spin $S$ can be written as

$$H(\boldsymbol{k})=v_1k_xS_x+v_2k_yS_y+v_3k_zS_z, \tag{S53}$$

where $v_i$ $(i=1,2,3)$ are band velocities and $S_a$ $(a=x,y,z)$ are matrices that satisfy a spin algebra

$$[S_i,S_j]=i\epsilon_{ijk}S_k,\quad \text{for any triple}(i,j,k), \tag{S54}$$

The energy dispersion is $\varepsilon_m(\boldsymbol{k})=mh=m\sqrt{v_1^2k_x^2+v_2^2k_y^2+v_3^2k_z^2}$, where $m=-S,\cdots,S$. The Berry curvature for the $m$-th band of this model is expressed as $\Omega_{m,a}=-mv_1v_2v_3k_a/h^3$ and, therefore, the Chern number of these bands is simply given by $\mathcal{C}_m=-2m\cdot\mathrm{sgn}(v_1v_2v_3)$. We now restrict ourselves to the $N=3$ and $N=4$ cases (i.e., to pseudospin-1 and pseudospin-3/2 fermions), which directly correspond to the multifold nodes in B20 compounds such as CoSi and PtAl.

### A. Pseudospin-1

After some detailed derivation, the BCP dipole for the model with $S=1$ is expressed as

$$\lambda_{xzz}(\boldsymbol{k})=\partial_xG_{zz}-\partial_zG_{xz}=\begin{pmatrix}\frac{2v_1^2v_3^2k_x}{h^5}\\ 0\\ -\frac{2v_1^2v_3^2k_x}{h^5}\end{pmatrix}. \tag{S55}$$

For the INPHE in the $x-z$ plane, the in-plane orbital magnetic moments are given by

$$\mathcal{M}_x^{\mathrm{O}}=\begin{pmatrix}-\frac{v_1v_2v_3k_x}{2h^2} & -\frac{v_2v_3\sqrt{2(v_2^2k_y^2+v_3^2k_z^2)}}{4h^2} & 0\\ \cdots & -\frac{v_1v_2v_3k_x}{h^2} & -\frac{v_2v_3\sqrt{2(v_2^2k_y^2+v_3^2k_z^2)}}{4h^2}\\ \cdots & \cdots & -\frac{v_1v_2v_3k_x}{2h^2}\end{pmatrix}, \tag{S56}$$

and

$$\mathcal{M}_z^{\mathrm{O}}=\begin{pmatrix}-\frac{v_1v_2v_3k_z}{2h^2} & \frac{i\sqrt{2}v_1v_2(v_1^2v_2k_x^2k_y+v_2^3k_y^3+v_2v_3^2k_yk_z^2-iv_1v_3k_xk_zh)}{4\sqrt{v_2^2k_y^2+v_3^2k_z^2}h^3} & 0\\ \cdots & -\frac{v_1v_2v_3k_z}{h^2} & \frac{i\sqrt{2}v_1v_2(v_1^2v_2k_x^2k_y+v_2^3k_y^3+v_2v_3^2k_yk_z^2-iv_1v_3k_xk_zh)}{4\sqrt{v_2^2k_y^2+v_3^2k_z^2}h^3}\\ \cdots & \cdots & -\frac{v_1v_2v_3k_z}{2h^2}\end{pmatrix}, \tag{S57}$$

with (...) indicating the Hermitian conjugate of the matrices. Note that the off-diagonal elements are no longer 0, which is different from the situation in the above two-band model with $S=1/2$.

The orbital magnetic susceptibility of BCP is given by

$$\Lambda_{zzx}^{\pm,\mathrm{O}}=\frac{3v_1v_2v_3^3k_x(v_1^2k_x^2+v_2^2k_y^2)}{2h^8}-\frac{v_1v_2v_3^5k_xk_z^2}{h^8}, \tag{S58}$$

$$\Lambda_{xzx}^{\pm,\mathrm{O}}=-\frac{3v_1^3v_2v_3^3k_x^2k_z}{2h^8}+\frac{v_1v_2v_3^3k_z(v_2^2k_y^2+v_3^2k_z^2-v_1^2k_x^2)}{2h^8}. \tag{S59}$$

Next, we derive the $xzzx$ element of the conductivity.

$$\alpha_{\mathrm{O}}^{\mathrm{I}}=\frac{|v_1v_2v_3^3|(-v_3^2k_z^2+3v_1^2k_x^2)}{2h^7}\mathrm{sgn}(v_1v_2v_3)\begin{pmatrix}-1\\0\\1\end{pmatrix}, \tag{S60}$$

$$\alpha_{\mathrm{O}}^{\mathrm{II}}=\frac{|v_1^3v_2v_3^3|k_x^2}{h^7}\mathrm{sgn}(v_1v_2v_3)\begin{pmatrix}-1\\0\\1\end{pmatrix}. \tag{S61}$$

We find that when $h$ is small, $\alpha_{\mathrm{O}}^{\mathrm{I/II}} \propto 1/h^5$ and depends on the chirality of the nodal point. After integral the produce of $f'$ and $\alpha$ in Eqs. (S60) and (S61), we can get:

$$\chi_{\mathrm{O}}^{\mathrm{I}} = \chi_{\mathrm{O}}^{\mathrm{II}} = -\frac{v_3^2 \operatorname{sgn}(v_1 v_2 v_3)}{6\pi^2\mu^3} = -\frac{v_3^2}{12\pi^2\mu^3}\mathcal{C}. \tag{S62}$$

which is distinct from the above case of $S = 1/2$. Consequently, the orbital contribution to the INPHE is about 8 times over that in the case of $S = 1/2$. For topological chiral semimetals such as CoSi, the 6-fold nodes at the corner of the first Brillouin zone (the R point) can be described by a *double* pseudospin-1 model with a Chern number of $\mathcal{C} = \pm 4$. Therefore, the INPHE induced by these 6-fold fermions is expected to be 16 times larger than the pseudo-spin-1/2 model with the same parameters.

### B. Pseudospin-3/2

Now we consider the four-band Hamiltonian (S53) with $S = 3/2$, which is also known as the Rarita–Schwinger–Weyl fermion. The energy spectrum contains four bands which are given by

$$\varepsilon(\boldsymbol{k}) = h \begin{pmatrix} -3/2 \\ -1/2 \\ 1/2 \\ 3/2 \end{pmatrix}, \tag{S63}$$

where $h = \sqrt{v_1^2 k_x^2 + v_2^2 k_y^2 + v_3^2 k_z^2}$. The BCP dipole is expressed as

$$\lambda_{xzz}(\boldsymbol{k}) = \frac{v_1^2 v_3^2 k_x}{h^5} \begin{pmatrix} 3 \\ 1 \\ -1 \\ -3 \end{pmatrix}. \tag{S64}$$

The diagonal elements of the orbital magnetic moment are given by

$$M_a = -\frac{v_1 v_2 v_3 k_a}{h^2} \begin{pmatrix} 3/4 \\ 7/4 \\ 7/4 \\ 3/4 \end{pmatrix}. \tag{S65}$$

Then we can get

$$\alpha_{\mathrm{O}}^{\mathrm{II}} = \frac{|v_1^3 v_2 v_3^3| k_x^2}{h^7} \operatorname{sgn}(v_1 v_2 v_3) \begin{pmatrix} -9/4 \\ -7/4 \\ 7/4 \\ 9/4 \end{pmatrix}, \tag{S66}$$

By integrating the produce of $f'$ and $\alpha$ in Eq. (S66), we arrive at

$$\chi_{\mathrm{O}}^{\mathrm{II}} = -\frac{11 v_3^2 \operatorname{sgn}(v_1 v_2 v_3)}{12\pi^2\mu^3} = -\frac{11 v_3^2}{36\pi^2\mu^3}\mathcal{C}. \tag{S67}$$

Due to the increased number of bands at this stage, $\alpha_{\mathrm{O}}^{\mathrm{I}}$ and $\chi_{\mathrm{O}}^{\mathrm{I}}$ cannot be expressed in simple terms. However, our numerical results indicate similar behavior of $\chi_{\mathrm{O}}^{\mathrm{I}}$ as the pseudospin-1 case. As shown in Fig. S1, the magnitudes of $\chi_{\mathrm{O}}^{\mathrm{I}}$ and $\chi_{\mathrm{O}}^{\mathrm{II}}$ are comparable, though the magnitude of $\chi_{\mathrm{O}}^{\mathrm{I}}$ is slightly larger, deviating from strict equality. Consequently, the INPHE induced by these 4-fold fermions is expected to be about 22 times larger than the pseudo-spin-1/2 model with the same parameters.

In summary, the INPHE is prominent when the chemical potential is tuned around nodal fermions in topological chiral semimetals. The INPHE response switches sign upon chirality reversal for chiral enantiomers with opposite handednesses. Moreover, multifold fermions that are described by the effective model with high pseudospin S can induce giant INPHE response. Compared to the INPHE of the pseudospin $S = 1/2$ case, the INPHE induced by the multifold degenerate nodes (which are characterized by pseudospin $S = 3/2$ or double pseudospin $S = 1$) at the R or $\Gamma$ points of B20 compounds would induce a significant INPHE which is about one order of magnitude larger than Weyl fermions with similar band velocities, as presented in Table S1.

Nevertheless, in practice, the experimentally measured peak values of INPHE in topological chiral crystals depend on the band velocity around the nodes, the relative energy of nodes with respect to the Fermi level, the temperature at which the experiment was conducted, and the sample quality of the chiral crystal.

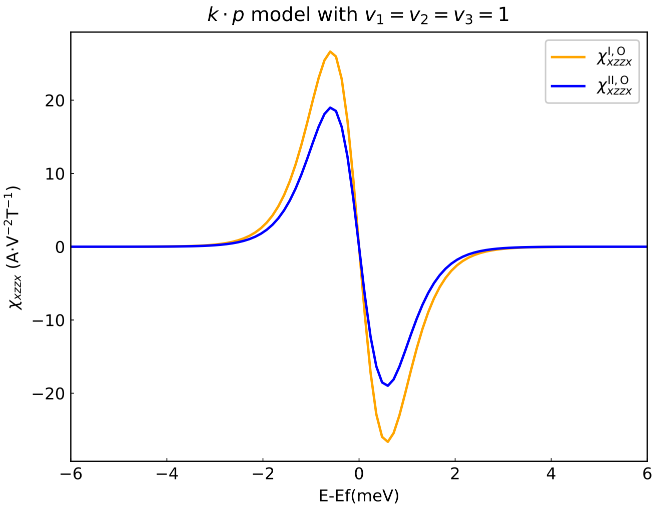


FIG. S1. Calculated response coefficient $\chi_{zxxz}$ versus the chemical potential $\mu$ for the k.p model with pseudospin $S = 3/2$. In the calculation, we take a $81 \times 81 \times 81$ k-mesh and the temperature is set to be $T = 5$ K.

TABLE S1. Comparison of the orbital part of INPHE induced by multifold fermions based on the k.p Hamiltonian (S53).

| Pseudospin | Chern number $\mathcal{C}$ | The INPHE conductivity $\chi^{\mathrm{O}}_{xzzx}$ | Material example |
|---|---|---|---|
| $S = 1/2$ | $\pm 1$ | $\chi^{\mathrm{I,O}}_{xzzx} = 0$, $\chi^{\mathrm{II,O}}_{xzzx} = -\frac{v_3^2}{24\pi^2\mu^3}\mathcal{C}$ | H point of Te |
| double $S = 1$ | $\pm 4$ | $\chi^{\mathrm{I,O}}_{xzzx} = \chi^{\mathrm{II,O}}_{xzzx} = -\frac{v_3^2}{12\pi^2\mu^3}\mathcal{C}$ | R point of CoSi |
| $S = 3/2$ | $\pm 4$ | $\chi^{\mathrm{I,O}}_{xzzx} \approx \chi^{\mathrm{II,O}}_{xzzx} = -\frac{11 v_3^2}{48\pi^2\mu^3}\mathcal{C}$ | $\Gamma$ point of CoSi |

## VI. FIRST-PRINCIPLES CALCULATION METHODS

We performed the first-principles calculations based on the density functional theory with the projector augmented wave method, as implemented in the Vienna *ab initio* simulation package (VASP) [20]. The generalized-gradient approximation in the form of the Perdew-Burke-Ernzerhof functional was employed for the exchange-correlation potential [21]. To obtain accurate band structures, we employed the Heyd-Scuseria-Ernzerhof (HSE) [22] hybrid functional in our calculations. The kinetic energy cutoff for plane wave expansion was set to 500 eV, and a $12 \times 12 \times 7$ **k**-mesh was used in all calculations. The Tkatchenko and Scheffler (DFT-TS) [23] van der Waals correction was adopted for better agreement of the optimized lattice parameters of Te with the experimental data [24]. The spin-orbit coupling (SOC) effect was taken into consideration for all electronic structure calculations. To calculate and band geometric quantities and obtain the INPHE conductivity, we generate *ab initio* tight-binding Hamiltonian based on atomically projected Wannier functions using the Wannier90 package [25]. Specifically, the Wannier functions are constructed by projecting the Bloch states onto Te-$s$ and Te-$p$ orbitals without applying a subsequent maximal-localization procedure. Then we take a $601 \times 601 \times 601$ k-mesh and set the temperature to $T = 5$ K for the integral in Eq. (**??**). To describe Te under strain, we apply a biaxial strain along the hexagonal plane of Te to preserve its hexagonal symmetry.

## VII. MORE CALCULATED RESULTS OF CHIRAL TE

More results of the right-handed Te are presented in Figs. S2-S7, including the other nonzero component of the INPHE conductivity $\chi_{zxxz}$, band-resolved BCP dipole $\lambda^n_{xzz} = \partial_x G^n_{zz} - \partial_z G^n_{xz}$, spin and orbital magnetic moment $\mathcal{M}^{n,\mathrm{S}}_x$ and $\mathcal{M}^{n,\mathrm{O}}_x$, and other band geometric quantities ($\alpha^{n,\mathrm{II,O}}, \alpha^{n,\mathrm{I,O}}$, and $\beta = \sum_n f'\alpha$) around the H point in momentum space.

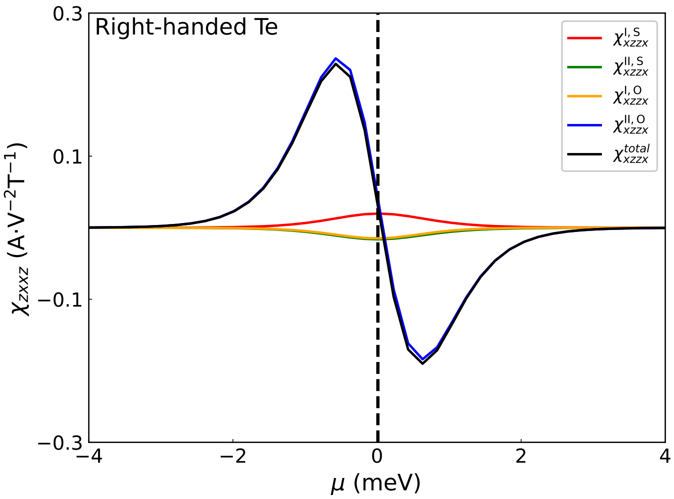


FIG. S2. Calculated response coefficient $\chi_{zxxz}$ versus the chemical potential $\mu$ for the right-handed Te. In the calculation, we take a $601 \times 601 \times 601$ k-mesh, and the temperature is set to be $T = 5$ K.

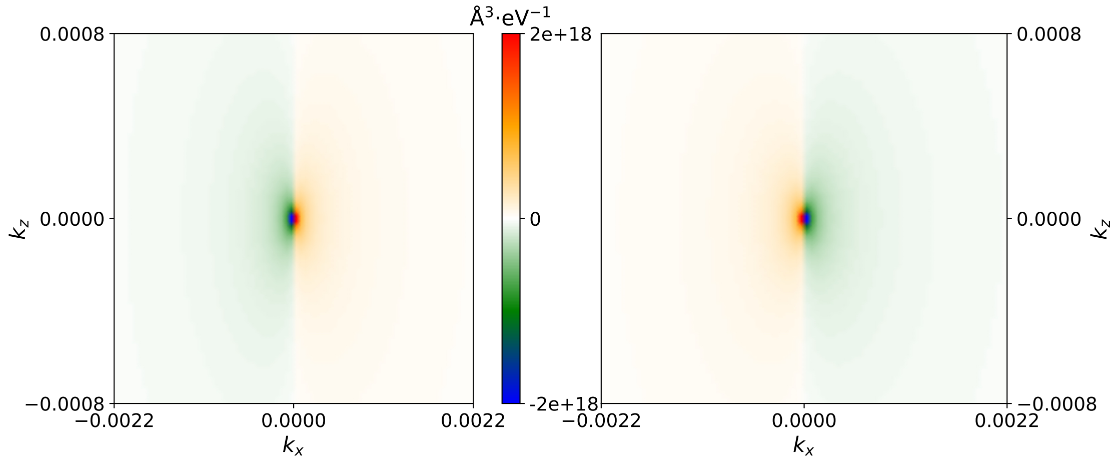


FIG. S3. The band-resolved $\lambda^n_{xzz} = \partial_x G^n_{zz} - \partial_z G^n_{xz}$ for the bottom two conduction bands ($n = 19$ and 20) of right-handed Te. The left and right panel corresponds to bands 19 and 20, respectively. The $\boldsymbol{k}$-plane shown here is the $k_x - k_z$-plane crossing the H point. The unit of $k_x$ and $k_z$ is Å$^{-1}$. The value of $\partial_x G^n_{zz} - \partial_z G^n_{xz}$ is opposite for the two bands. To achieve a clear and intuitive display of the data, the heatmap is plotted using the fourth power transformation of the original data: $\lambda^{1/4}$.

We have presented the results of right-handed Te under a biaxial strain of 3% in Fig. 3(d-f) in the main text. Figure S8 shows the k-space distribution of relevant band geometric quantities around the new WPs induced by the strain.

By further increasing the strain, chiral Te undergoes an insulator-semimetal transition with multiple Weyl nodes appearing near the Fermi level. As shown in Fig. S9, under a 9% biaxial strain, the highest valence band is pushed up and intersects with the conduction bands, creating 4 WPs in the H-K line (along the $k_z$ direction). Interestingly, one observes giant INHPE peaks on the order of $10^1 \sim 10^2 \mathrm{A} \cdot \mathrm{V}^{-2} \cdot \mathrm{T}^{-1}$ around these new WPs, which are quite large and detectable in experiments. Moreover, these peaks are mainly contributed by $\chi^{\mathrm{II,O}}$ due to the large band velocity $v_3$ along $k_z$ direction and small tilt of these strain-induced Weyl fermions.

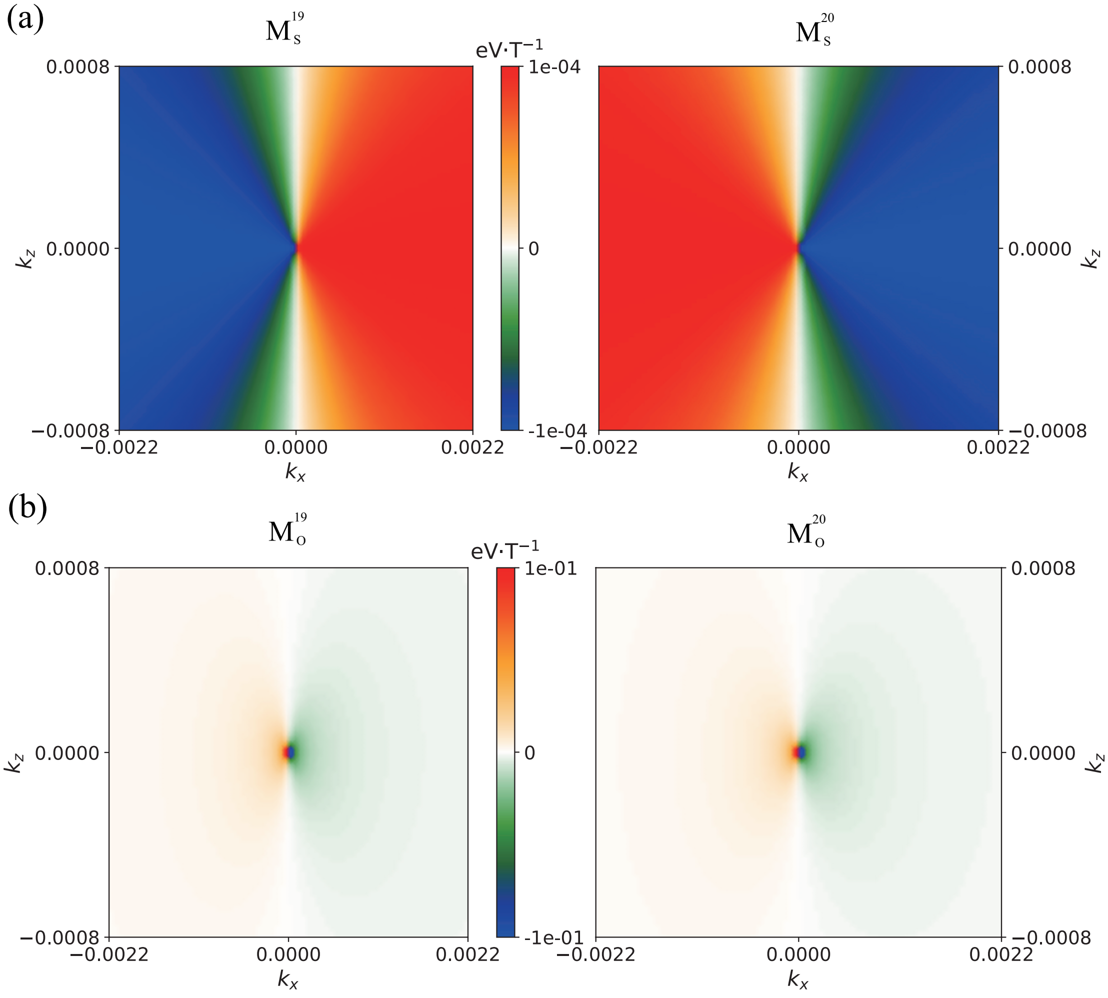


FIG. S4. (a,b) The band-resolved $\mathcal{M}_x^{n,\mathrm{S}}$ and $M_x^{n,\mathrm{O}}$ for the bottom two conduction bands ($n = 19$ and 20) of right-handed Te. The $\boldsymbol{k}$-plane shown here is the $k_x - k_z$-plane crossing the H point. The unit of $k_x$ and $k_z$ is Å$^{-1}$. The unit of $k_x$ and $k_z$ is Å$^{-1}$. Both the spin and orbital moments are odd functions of $k_x$. $\mathcal{M}_x^{n,\mathrm{S}}$ is opposite for the two bands, while $\mathcal{M}_x^{n,\mathrm{O}}$ is the same. $\mathcal{M}_x^{n,\mathrm{O}}$ is more sensitive to the decreasing local gap around the WP.

## VIII. TOPOLOGICAL CHIRAL SEMIMETALS WITH MULTIFOLD FERMIONS (COSI, RHSI, RHSN, PTGA, AND PTAL)

We present the results of B20 compounds in Figs. S10-S14, including left- and right-handed CoSi, right-handed RhSi, RhSn, PtAl, and PtGa.

The B20 compounds AB (A = Co, Rh, Pt; B = Si, Sn, Ga, Al) have chiral cubic structures with the space group $P2_13$ (No.198), which contains two main symmetry operations: a three-fold rotation about the [111] direction and a nonsymmorphic screw symmetry that combines a two-fold rotation about the z-axis with a translation by (1/2, 0, 1/2). The combination of these symmetry operations gives rise to three nonintersecting two-fold screw rotations along the $x$, $y$, and $z$ axes and four three-fold rotations along the cube's main diagonals. Due to the symmetry constraint, the allowed components of NPHE are $\chi_{abba}$ with $a, b = x, y, z$. Taking CoSi as an example, the right-handed chiral crystals are defined as the Co and Si atoms forming right and left helices in the view of [111] direction, as shown in Fig. S10(a). Inversely, the left-handed chiral crystal is formed when Co and Si atoms form left- and right-handed helices, respectively.

As shown in Fig. S10(b), there is a fourfold degenerate band crossing at the $\Gamma$ point and a six-fold one at the R point of the first Brillouin zone. The magnitude of the Chern number for these nodes is limited to $|\mathcal{C}| = 4$, the sign depends on the structural chirality of their host crystal: $\mathcal{C} = +4$ at $\Gamma$ and $\mathcal{C} = -4$ at R for the left-handed CoSi, and they reverse sign upon chirality reversal.

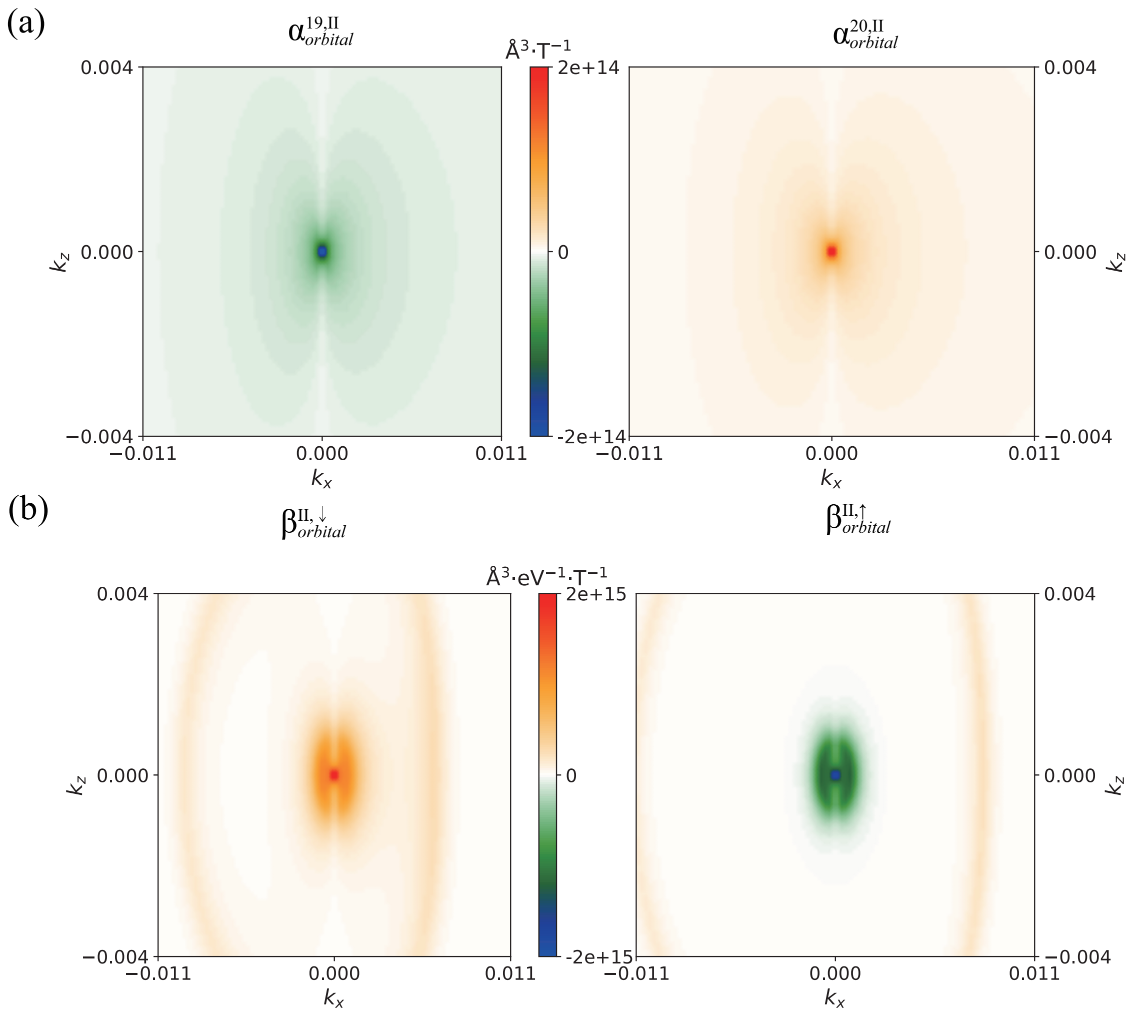


FIG. S5. (a) The k-resolved $\alpha^{n,\mathrm{II,O}}_{xzzx}$ for the bottom two conduction bands ($n$ = 19 and 20) of the right-handed Te. (b) The k-resolved $\beta^{\mathrm{II,O}}_{xzzx} = \sum_n f' \alpha^{n,\mathrm{II,O}}_{xzzx}$ of right-handed Te, where the $\mu$ is 0.4 meV below (above) the Weyl node for ↓ (↑). The k-plane is the same as the above figures. To achieve a clear and intuitive display of the data, the heatmap is plotted using the sixth power transformation of the original data: $\alpha^{1/6}$.

TABLE S2. Band velocity $v_3$ (eV·Å) around Γ and R for the five B20 compounds. The values are obtained by fitting the effective model (S53) with the first-principles band structures around Γ and R.

| Material | $\lvert v_3 \rvert$ at Γ (eV·Å) | $\lvert v_3 \rvert$ at $R$ (eV·Å) |
|---|---|---|
| CoSi | 0.786 | 0.903 |
| RhSi | 1.223 | 1.633 |
| RhSn | 0.837 | 1.296 |
| PtGa | 1.723 | 1.701 |
| PtAl | 2.095 | 1.934 |

Inspection of the results in Fig. S10-S14 reversals that all five topological chiral semimetals show large amplitudes of INPHE which are at least one order of magnitude larger than that of chiral Te. This indicates that multifold nodal fermions with high Chern numbers indeed lead to significant INPHE, which facilitates experimental measurements of INPHE in these materials. Among all these compounds we studied, PtAl is the most promising candidate for detecting the giant INPHE conductivity, as the calculated peak value of $\chi_{xzzx}$ reaches about 20 A · V$^{-2}$ · T$^{-1}$. Comparing the band velocity parameter from the first-principles band structure (as listed in Table. S2), we conclude that the large INHPE of PtAl is mainly due to the large band velocity.

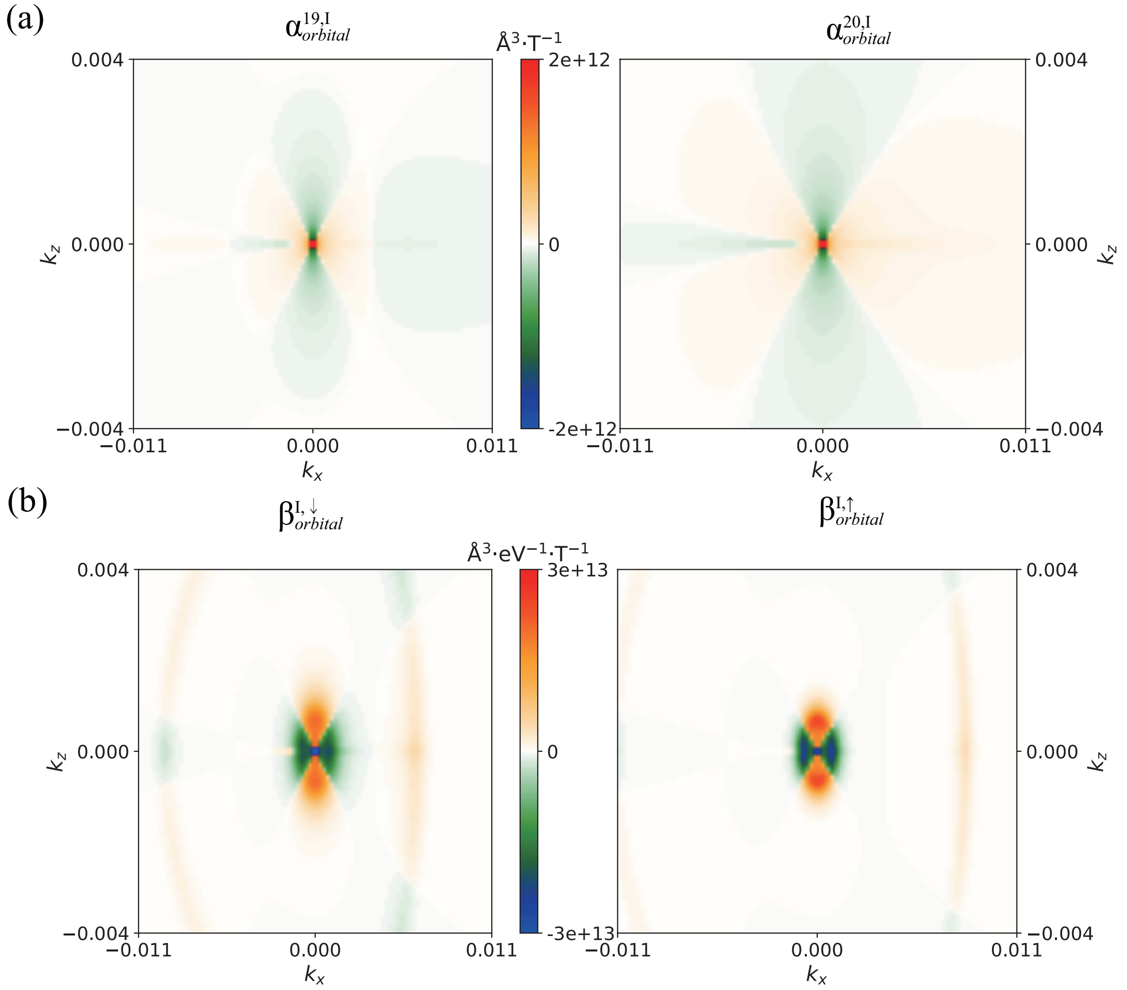


FIG. S6. (a) The k-resolved $\alpha^{n,\mathrm{I,O}}_{xzzx}$ for the bottom two conduction bands ($n$ = 19 and 20) of the right-handed Te. (b) The k-resolved $\beta^{\mathrm{I,O}}_{xzzx} = \sum_n f' \alpha^{n,\mathrm{I,O}}_{xzzx}$ of right-handed Te, where the $\mu$ is 0.4 meV below (above) the Weyl node for $\downarrow$ ($\uparrow$). The k-plane is the same as the above figures. To achieve a clear and intuitive display of the data, the heatmap is plotted using the power transformation of the original data: $\alpha^{1/3.6}$.

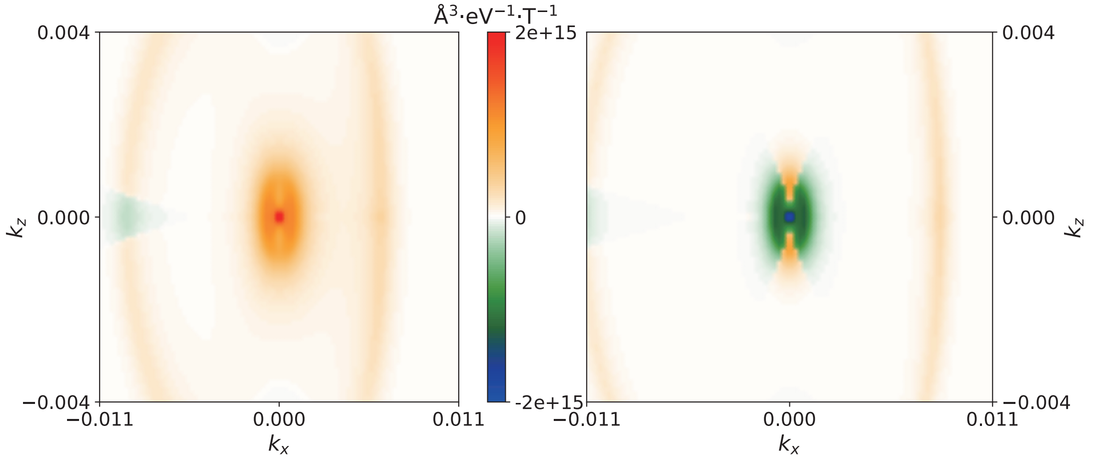


FIG. S7. (a) The k-resolved $\beta^{\mathrm{O}}_{xzzx} = \beta^{\mathrm{I,O}}_{xzzx} + \beta^{\mathrm{II,O}}_{xzzx}$ for the bottom two conduction bands ($n$ = 19 and 20) of the right-handed Te, where the $\mu$ is 0.4 meV below (above) the Weyl node for $\downarrow$ ($\uparrow$). The k-plane is the same as the above figures. To achieve a clear and intuitive display of the data, the heatmap is plotted using the sixth power transformation of the original data: $\beta^{1/6}$.

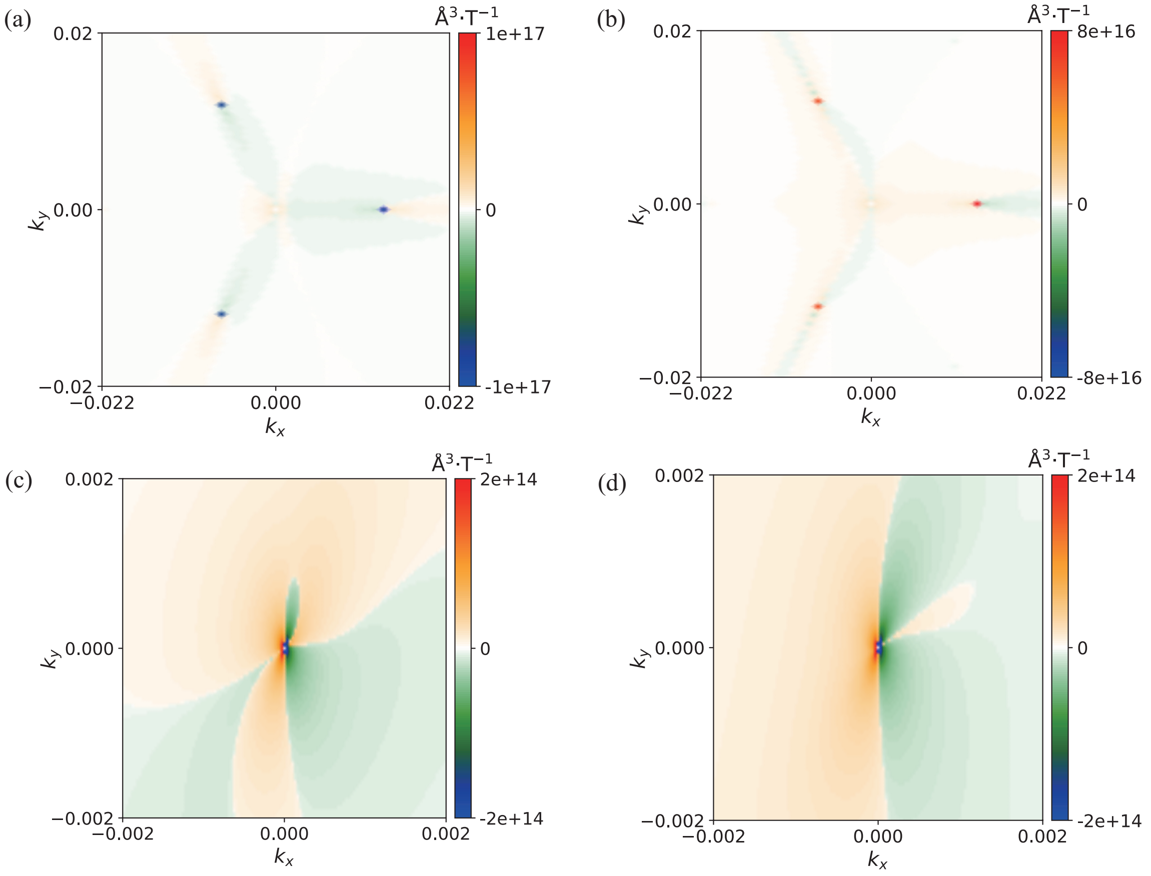


FIG. S8. (a,b) $\alpha^{\mathrm{I,O}}$ for the 19-th and 20-th band in $k_x$-$k_y$ plane crossing H. (c,d) $\alpha^{\mathrm{I,O}}$ for the 19-th and 20-th band in the $k_y$-$k_z$ plane crossing the WP $W_3$ labeled in Fig. 3(e). The left and right panels are for the 19-th and 20-th bands, respectively.

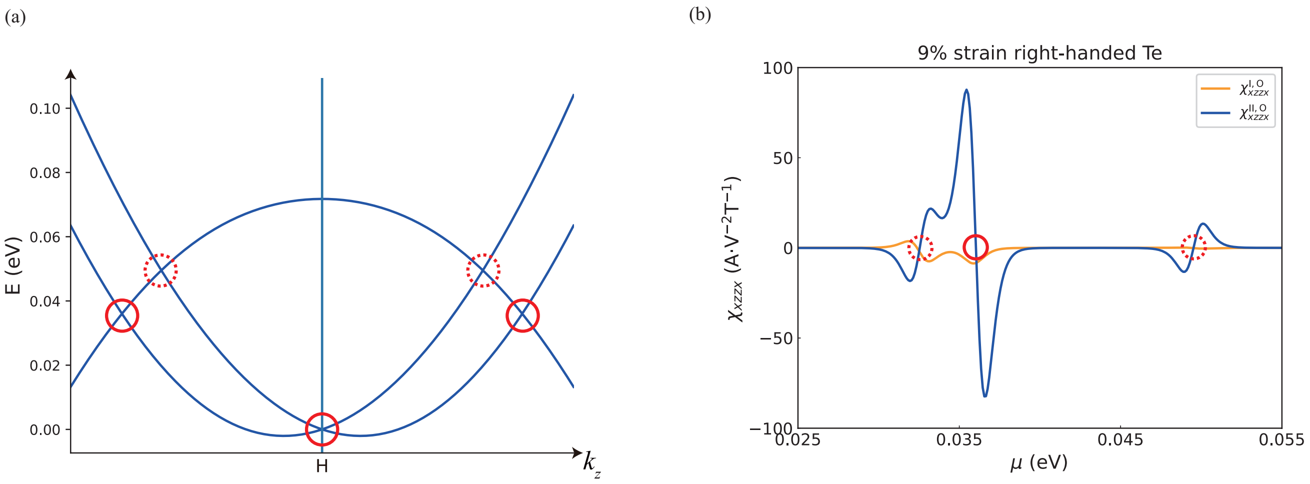


FIG. S9. (a) The band structure along $k_z$ near the WP at H for the right-handed Te under biaxial in-plane strain of 9%. The solid (dashed) circle represents Weyl node with +1(-1) chirality. (b) Calculated response coefficient $\chi_{zxxz}$ versus the chemical potential $\mu$ for the strained Te.

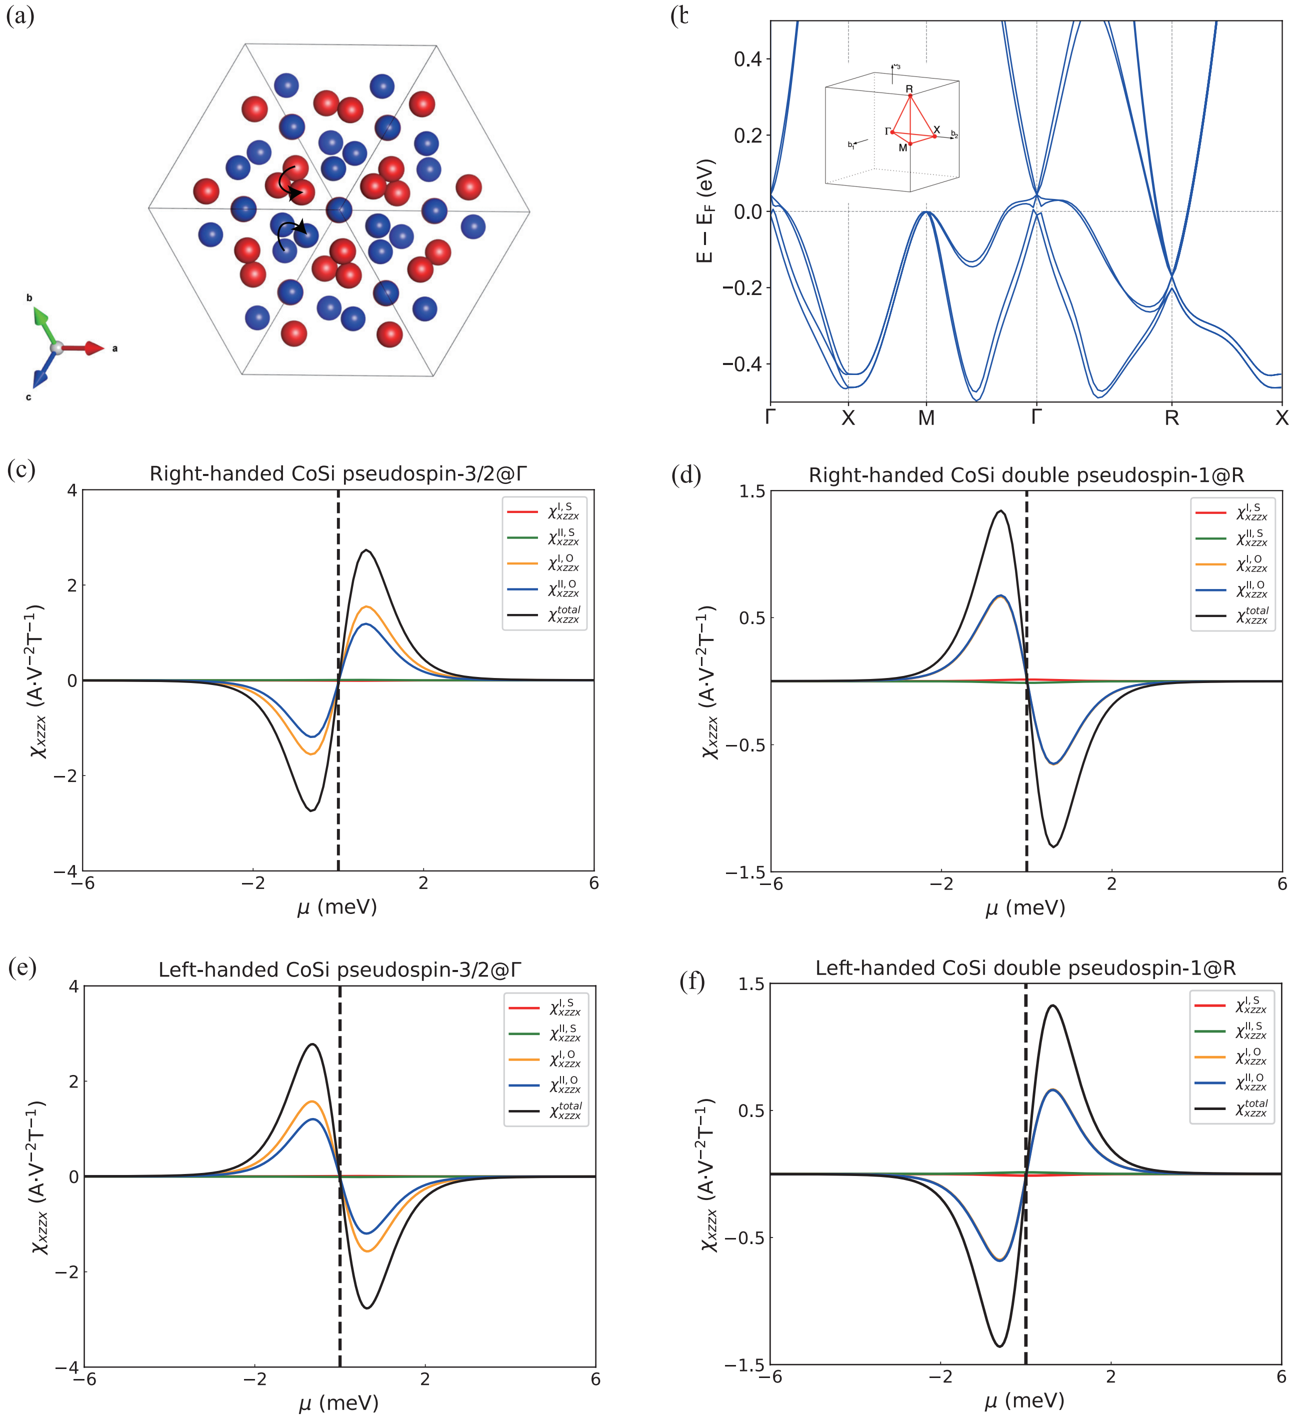


FIG. S10. (a) The crystal structure of the B20 compounds AB (A=Co, Rh, Pt; B=Si, Sn, Ga, Al). The right-handed (left-handed) chiral crystal is represented by this structure when the red (blue) atomic positions are occupied by A (i.e., Co, Rh, or Pt). (b) Band structure of the right-handed CoSi. (c,e) Calculated response coefficient $\chi_{xzzx}$ versus the chemical potential $\mu$ for the right- and left-handed CoSi around the fourfold-degenerate point at Γ. (d,f) Calculated response coefficient $\chi_{xzzx}$ versus the chemical potential $\mu$ for the right- and left-handed CoSi around the sixfold-degenerate point at R.

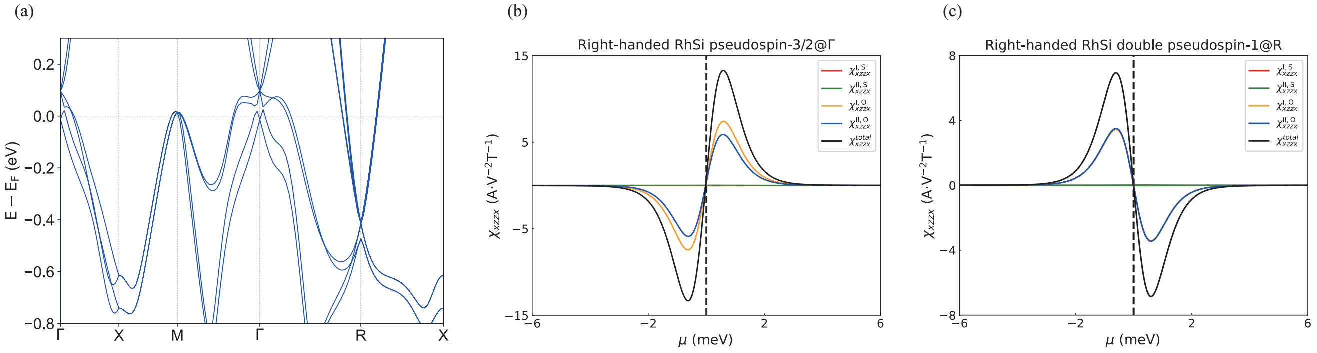


FIG. S11. (a) Band structure of right-handed RhSi. (b,c) Calculated response coefficient $\chi_{xzzx}$ versus the chemical potential $\mu$ for the right-handed RhSi around the fourfold-degenerate point at $\Gamma$ and the sixfold-degenerate point at R, respectively.

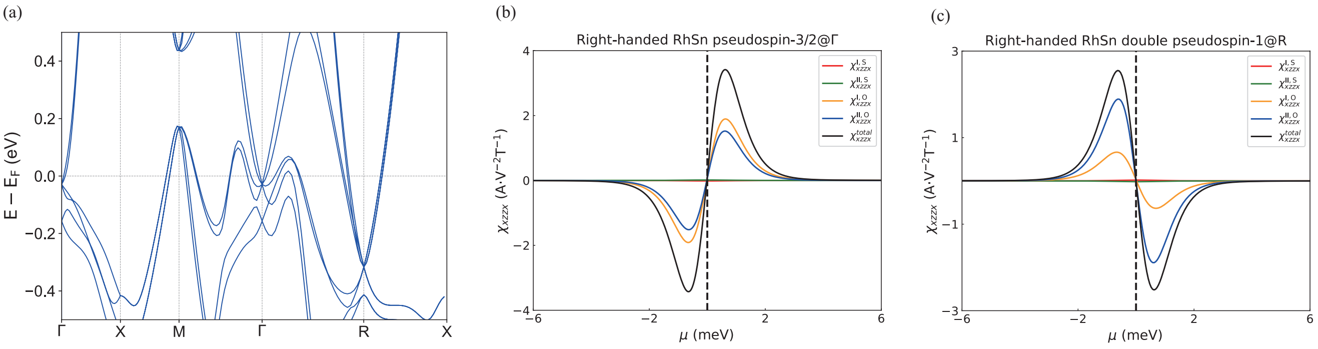


FIG. S12. (a) Band structure of right-handed RhSn. (b,c) Calculated response coefficient $\chi_{xzzx}$ versus the chemical potential $\mu$ for the right-handed RhSn around the fourfold-degenerate point at $\Gamma$ and the sixfold-degenerate point at R, respectively.

---


[1] H. Liu, J. Zhao, Y.-X. Huang, W. Wu, X.-L. Sheng, C. Xiao, and S. A. Yang, Intrinsic second-order anomalous Hall effect and its application in compensated antiferromagnets, Phys. Rev. Lett. **127**, 277202 (2021).

[2] C. Wang, Y. Gao, and D. Xiao, Intrinsic nonlinear Hall effect in antiferromagnetic tetragonal CuMnAs, Phys. Rev. Lett. **127**, 277201 (2021).

[3] J. Wang, H. Zeng, W. Duan, and H. Huang, Intrinsic nonlinear Hall detection of the néel vector for two-dimensional antiferromagnetic spintronics, Phys. Rev. Lett. **131**, 056401 (2023).


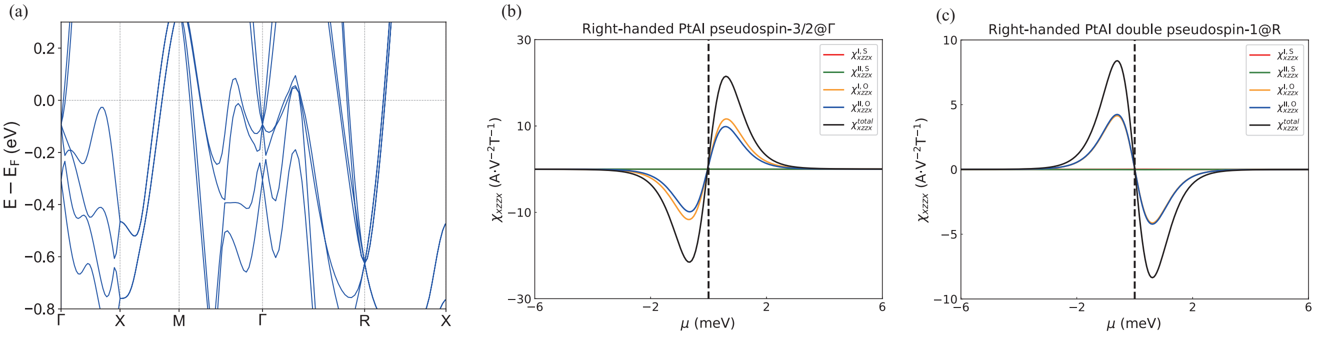


FIG. S13. (a) Band structure of right-handed PtAl. (b,c) Calculated response coefficient $\chi_{xzzx}$ versus the chemical potential $\mu$ for the right-handed PtAl around the fourfold-degenerate point at $\Gamma$ and the sixfold-degenerate point at R, respectively.

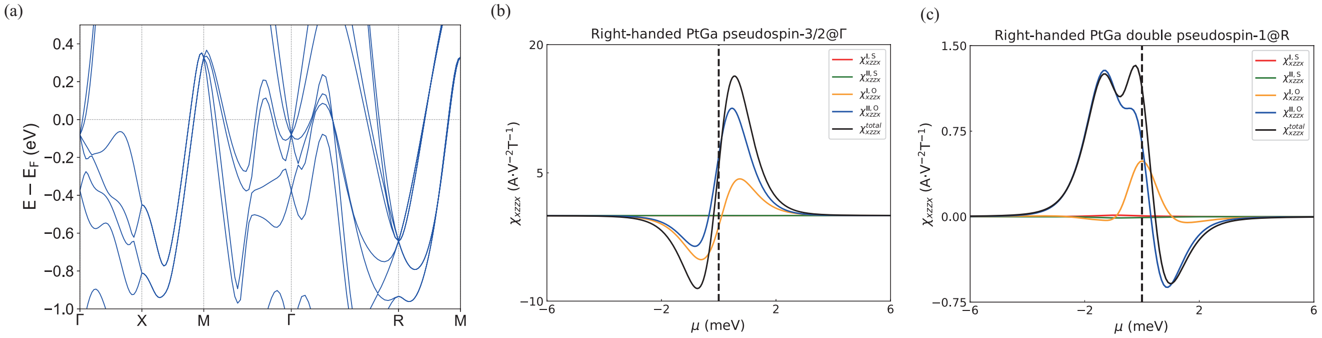


FIG. S14. (a) Band structure of right-handed PtGa. (b,c) Calculated response coefficient $\chi_{xzzx}$ versus the chemical potential $\mu$ for the right-handed PtGa around the fourfold-degenerate point at Γ and the sixfold-degenerate point at R, respectively.


[4] T. Doi, K. Nakao, and H. Kamimura, The valence band structure of tellurium. i. the k·p perturbation method, J. Phys. Soc. Japan **28**, 36 (1970).

[5] T. Furukawa, Y. Watanabe, N. Ogasawara, K. Kobayashi, and T. Itou, Current-induced magnetization caused by crystal chirality in nonmagnetic elemental tellurium, Phys. Rev. Res. **3**, 023111 (2021).

[6] M. Hirayama, R. Okugawa, S. Ishibashi, S. Murakami, and T. Miyake, Weyl node and spin texture in trigonal tellurium and selenium, Phys. Rev. Lett. **114**, 206401 (2015).

[7] G. L. Bir and G. E. Pikus, *Symmetry and strain-induced effects in semiconductors*, Vol. 624 (Wiley, New York, 1974).

[8] T. Kikuchi, T. Koretsune, R. Arita, and G. Tatara, Dzyaloshinskii-moriya interaction as a consequence of a doppler shift due to spin-orbit-induced intrinsic spin current, Phys. Rev. Lett. **116**, 247201 (2016).

[9] D. Gosálbez-Martínez, A. Crepaldi, and O. V. Yazyev, Diversity of radial spin textures in chiral materials, Phys. Rev. B **108**, L201114 (2023).

[10] C. Niu, G. Qiu, Y. Wang, P. Tan, M. Wang, J. Jian, H. Wang, W. Wu, and P. D. Ye, Tunable chirality-dependent nonlinear electrical responses in 2d tellurium, Nano Lett. **23**, 8445 (2023).

[11] G. Gatti, D. Gosálbez-Martínez, S. S. Tsirkin, M. Fanciulli, M. Puppin, S. Polishchuk, S. Moser, L. Testa, E. Martino, S. Roth, P. Bugnon, L. Moreschini, A. Bostwick, C. Jozwiak, E. Rotenberg, G. Di Santo, L. Petaccia, I. Vobornik, J. Fujii, J. Wong, D. Jariwala, H. A. Atwater, H. M. Rønnow, M. Chergui, O. V. Yazyev, M. Grioni, and A. Crepaldi, Radial spin texture of the Weyl fermions in chiral tellurium, Phys. Rev. Lett. **125**, 216402 (2020).

[12] G. Qiu, C. Niu, Y. Wang, M. Si, Z. Zhang, W. Wu, and P. D. Ye, Quantum hall effect of Weyl fermions in n-type semiconducting tellurene, Nat. Nanotechnol. **15**, 585 (2020).

[13] Y. Wang, G. Qiu, R. Wang, S. Huang, Q. Wang, Y. Liu, Y. Du, W. A. Goddard, M. J. Kim, X. Xu, P. D. Ye, and W. Wu, Field-effect transistors made from solution-grown two-dimensional tellurene, Nat. Electron. **1**, 228 (2018).

[14] K. F. Kang, T. X. Li, E. Sohn, J. Shan, and K. F. Mak, Nonlinear anomalous Hall effect in few-layer $WTe_2$, Nat. Mater. **18**, 324 (2019).

[15] J. Duan, Y. Jian, Y. Gao, H. Peng, J. Zhong, Q. Feng, J. Mao, and Y. Yao, Giant second-order nonlinear Hall effect in twisted bilayer graphene, Phys. Rev. Lett. **129**, 186801 (2022).

[16] P. He, S. S.-L. Zhang, D. Zhu, S. Shi, O. G. Heinonen, G. Vignale, and H. Yang, Nonlinear planar Hall effect, Phys. Rev. Lett. **123**, 016801 (2019).

[17] W. Rao, Y.-L. Zhou, Y.-j. Wu, H.-J. Duan, M.-X. Deng, and R.-Q. Wang, Theory for linear and nonlinear planar Hall effect in topological insulator thin films, Phys. Rev. B **103**, 155415 (2021).

[18] R. Battilomo, N. Scopigno, and C. Ortix, Anomalous planar Hall effect in two-dimensional trigonal crystals, Phys. Rev. Res. **3**, L012006 (2021).

[19] C. Niu, S. Huang, N. Ghosh, P. Tan, M. Wang, W. Wu, X. Xu, and P. D. Ye, Tunable circular photogalvanic and photovoltaic effect in 2d tellurium with different chirality, Nano Lett. **23**, 3599 (2023), pMID: 37057864.

[20] G. Kresse and J. Furthmüller, Efficiency of ab-initio total energy calculations for metals and semiconductors using a plane-wave basis set, Comput. Mater. Sci. **6**, 15 (1996).

[21] J. P. Perdew, K. Burke, and M. Ernzerhof, Generalized gradient approximation made simple, Phys. Rev. Lett. **77**, 3865 (1996).

[22] J. Heyd, G. E. Scuseria, and M. Ernzerhof, Hybrid functionals based on a screened coulomb potential, J. Chem. Phys. **118**, 8207 (2003).

[23] A. Tkatchenko and M. Scheffler, Accurate molecular van der waals interactions from ground-state electron density and free-atom reference data, Phys. Rev. Lett. **102**, 073005 (2009).

[24] X. Huang, J. Guan, Z. Lin, B. Liu, S. Xing, W. Wang, and J. Guo, Epitaxial growth and band structure of te film on graphene, Nano Lett. **17**, 4619 (2017).

[25] N. Marzari, A. A. Mostofi, J. R. Yates, I. Souza, and D. Vanderbilt, Maximally localized Wannier functions: Theory and applications, Rev. Mod. Phys. **84**, 1419 (2012).
